# Supplementary material for: Pointer Life Cycle Types for Lock-Free Data Structures with Memory Reclamation
Source: arXiv:1910.11714 source file (2019-11-26)
Supplement: Supplementary file 1 [file obs2nfa_proofs.tex]

%!TEX root = ../main.tex

\presection
\subsection{Observer to NFA}

\begin{proof}[Proof of \Cref{thm:observer-runs-vs-nfa-runs}]
	Consider some observer $\anobs$ and its abstraction $\anaut=\alpha(\anobs)$.
	To establish the claim, we consider single steps for some event $\anevent=f(\vecof{\aval})$ with $\vecof{\aval}=\aval[1],\dots,\aval[k]$.
	The overall claim then follows from induction.

	First, let $(\alocation_1,\varphi)\trans{\anevent}(\alocation_2,\varphi)$ be some step of $\anobs$.
	We show that $\anaut$ can do the step $\alocation_1^\sharp\trans{\alpha_\varphi(\anevent)}\alocation_2^\sharp$.
	By definition, we know that $\anobs$ contains a transition of the form $\alocation_1\trans{f(\vecof{r}),\aguard}\alocation_2$.
	Moreover, we know that this transition is enabled for $\anevent$, that is, we have $\varphi(\renamingof{\aguard}{\vecof{r}}{\vecof{\aval}})=\mathit{true}$.
	Let $\avals[i]:=\alpha_\varphi(\aval[i])$.
	It suffices to show that $(\avals[1],\dots,\avals[k])\in R^\sharp$ holds in order to establish the existence of the desired transition in $\anaut$.
	To that end, let $\Delta$ be a valuation such that $\Delta(r_i)=v_i$ and $\Delta(\anovar_i)=\varphi(\anovar_i)$.
	We show that $\Delta$ is a witness valuation for the satisfiability:
	\begin{align*}
		\phi\equiv
		\aguard
		~\wedge~
		\left(
		\bigwedge_{i\vphantom{i^\sharp}}
		\bigwedge_{\anovars_j\in\avals[i]} r_i=\anovar_j
		\right)
		~\wedge~
		\left(
		\bigwedge_{i\vphantom{i^\sharp}}
		\bigwedge_{\anovars_j\notin\avals[i]} r_i\neq\anovar_j
		\right)
		\ .
	\end{align*}
	Note that $\varphi(\renamingof{\aguard}{\vecof{r}}{\vecof{\aval}})=\mathit{true}$ implies $\Delta(\aguard)=\mathit{true}$.
	The remaining conjuncts of $\phi$ are in order.
	Consider some $i$ and some $j$.
	First, consider the case $\anovars_j\in\avals[i]$.
	This means $\anovars_j\in\alpha_\varphi(\aval[i])$.
	By definition, we get $\varphi(\anovar_j)=\aval[i]$.
	Hence, $\Delta(r_i=\anovar_j)=\mathit{true}$.
	Second, consider the case $\anovars_j\notin\avals[i]$.
	Towards a contradiction, assume $\varphi(\anovar_j)=\aval[i]$.
	Then, $\anovars_j\in\alpha_\varphi(\aval[i])$ follows by definition.
	Hence, $\anovars_j\in\avals[i]$.
	Since this contradicts the assumption, we must have $\anovars_j\notin\avals[i]$.
	So, $\Delta(r_i\neq\anovar_j)=\mathit{true}$.
	Altogether, we arrive at $\Delta(\phi)=\mathit{true}$.
	As desired, this entails the existence of $\alocation_1^\sharp\trans{\alpha_\varphi(\anevent)}\alocation_2^\sharp$ in $\anaut$ because $\alpha_\varphi(\anevent)=f(\avals[1],\dots,\avals[k])$.

	Now, let $\alocation_1^\sharp\trans{\alpha_\varphi(\anevent)}\alocation_2^\sharp$ be some step of $\anaut$.
	We show that $\anobs$ can take the step $(\alocation_1,\varphi)\trans{\anevent}(\alocation_2,\varphi)$.
	Note that $\alpha_\varphi(\anevent)=f(\avals[1],\dots,\avals[k])$.
	By definition of $\alpha(\anobs)=\anaut$, $\anobs$ contains a transition of the form $\alocation_1\trans{f(r_1,\dots,r_k),\aguard}\alocation_2$ such that $\satisfiableof{\phi}$ holds for:
	\begin{align*}
		\phi\equiv
		\aguard
		~\wedge~
		\left(
		\bigwedge_{i\vphantom{i^\sharp}}
		\bigwedge_{\anovars_j\in\avals[i]} r_i=\anovar_j
		\right)
		~\wedge~
		\left(
		\bigwedge_{i\vphantom{i^\sharp}}
		\bigwedge_{\anovars_j\notin\avals[i]} r_i\neq\anovar_j
		\right)
		\ .
	\end{align*}
	We now show that $\varphi(\aguard[\vecof{r}\mapsto\vecof{\aval}])=\mathit{true}$.
	Recall that $\aguard$ is conjunction over clauses $c_k$, $\aguard=\bigwedge_k c_k$.
	It suffices to show that $\varphi(c_k[\vecof{r}\mapsto\vecof{\aval}])=\mathit{true}$ for all clauses $c_k$.
	To that end, consider some clause $c_k$.
	We do a case distinction over its structure.
	\begin{compactenum}
		\item
			Consider the case $c_k\equiv r_i=\anovar_j$.
			We have to show that $\varphi(\anovar_j)=\aval[i]$ holds.
			Note that $\satisfiableof{\phi\wedge c_k}$ holds by definition.
			Hence, we must have $\anovars_j\in\avals[i]$ as for otherwise $\phi$ would contain $r_i\neq\anovar_j$ contradicting $\satisfiableof{\phi\wedge c_k}$.
			That is, $\anovars_j\in\alpha_\varphi(\aval[i])$.
			By definition, this means $\varphi(\anovar_j)=\aval[i]$ as desired.

		\item
			Consider the case $c_k\equiv r_i\neq\anovar_j$.
			We have to show that $\varphi(\anovar_j)\neq\aval[i]$ holds.
			Note that $\satisfiableof{\phi\wedge c_k}$ holds by definition.
			Hence, we must have $\anovars_j\notin\avals[i]$ as for otherwise $\phi$ would contain $r_i=\anovar_j$ contradicting $\satisfiableof{\phi\wedge c_k}$.
			That is, $\anovars_j\notin\alpha_\varphi(\aval[i])$.
			By definition, this means $\varphi(\anovar_j)\neq\aval[i]$ as desired.
	\end{compactenum}
	\notei{We cannot handle clauses of the form $r_i=r_j$ and $u_i=u_j$.}
	Altogether, we get that $\varphi(\aguard[\vecof{r}\mapsto\vecof{\aval}])=\mathit{true}$ holds as desired.
\end{proof}

\begin{proof}[Proof of \Cref{thm:nonempty-history-concretisation}]
	Let $\anobs$ be some observer, $\anaut=\alpha(\anobs)$ its abstraction, and let $\varphi$ be some observer variable valuation.
	Consider some abstract event $\anevent^\sharp\in\langof{\anaut}$.
	We show that there is a concrete history $\anevent$ such that $\anevent^\sharp=\alpha_\varphi(\anevent)$ holds.
	The abstract event $\anevent^\sharp$ is of the form $\anevent^\sharp=f(\avals[1],\dots,\avals[k])$.
	Let $\aval[i]$ be some concrete value such that $\avals[i]=\alpha_\varphi(\aval[i])$.
	Such $\aval[i]$ is guaranteed to exists.
	If $\avals[i]=\emptyset$, then $\aval[i]\notin\rangeof{\varphi}$.
	Note here that $\rangeof{\varphi}$ is finite.
	If $\avals[i]\neq\emptyset$, then there is $\anovars_j\in\avals[i]$.
	So choose $\aval[i]=\varphi(\anovars_j)$.
	Altogether, this means there are $\aval[1],\dots,\aval[k]$ such that \[ \alpha_\varphi(f(\aval[1],\dots,\aval[k]))=f(\avals[1],\dots,\avals[k]) \ . \]
	Applying the argument inductively to an entire history $\ahist^\sharp$ establishes the overall claim.
\end{proof}

\begin{proof}[Proof of \Cref{thm:concrete-vs-abstract-induced-histories}]
	First, consider $\ahist\in\typehistof{\athread}{\anadr}{\atype}$.
	That is, $\ahist\in\typehistof{\athread}{\anadr}{\aguarantee_i}$ for all $1\leq i\leq k$.
	So for every $\aguarantee_i$ there is a run $(\alocation_1,\varphi)\trans{\ahist}(\alocation_2,\varphi)$ where $\alocation_1$ is initial and $\alocation_2$ is final in $\anobs[i]$.
	Let $\anaut[i]=\alpha(\anobs[i])$.
	By \Cref{thm:observer-runs-vs-nfa-runs}, we have $\alpha_\varphi(\ahist)\in\langof{\anaut[i]}$.
	Altogether, we get $\alpha_\varphi(\ahist)\in\langof{\anaut[1]\times\cdots\times\anaut[k]}$ as desired.

	Second, consider $\alpha_\varphi(\ahist)\in\langof{\alpha(\anobs[1])\times\cdots\times\alpha(\anobs[k])}$.
	That is, $\alpha_\varphi(\ahist)\in\langof{\alpha(\anobs[i])}$ for all $1\leq i\leq k$.
	So for every $i$ there is a run $\alocation_1^\sharp\trans{\alpha_\varphi(\ahist)}\alocation_2^\sharp$ where $\alocation_1^\sharp$ is initial and $\alocation_2^\sharp$ is final in $\alpha(\anobs[i])$.
	From \Cref{thm:observer-runs-vs-nfa-runs} we get the run $(\alocation_1,\varphi)\trans{\ahist}(\alocation_2,\varphi)$ of $\anobs[i]$.
	So, $\ahist\in\typehistof{\athread}{\anadr}{\aguarantee_i}$.
	Altogether, this gives $\ahist\in\typehistof{\athread}{\anadr}{\atype}$ as desired.
\end{proof}

\begin{proof}[Proof of \Cref{thm:type-inference-via-nfas}]
	Consider some types $\atype,\atypep\typefrom\aninstantiation$.
	Let $\anevent$ be some event, $\athread$ some thread, and $\anadr$ some address.
	Let $\varphi=\set{\anovar\mapsto\athread,\anovarp\mapsto\anadr}$.
	Assume that for every guarantee $\aguarantee$ available in $\aninstantiation$ we have some observer $\anobs[\aguarantee]$ such that $\typehistof{\athread}{\anadr}{\aguarantee}=\setcond{\ahist}{\exists\alocation_1,\alocation_2.~(\alocation_1,\varphi)\trans{\ahist}(\alocation_2,\varphi)\text{ with $\alocation_1$ initial and $\alocation_2$ final in $\anobs[\aguarantee]$}}$.
	Choose the following automata:
	\begin{compactitem}
		\item $\anaut[1]:=\bigcap\setcond{\alpha(\anobs[\aguarantee])}{\aguarantee\in\atype}$
		\item $\anaut[2]$ such that $\langof{\anaut[2]}=\set{\alpha_\varphi(\anevent)}$.
		\item $\anaut$ such that $\langof{\anaut}=\setcond{\ahist_1^\sharp.\ahist_2^\sharp}{\ahist_1^\sharp\in\langof{\anaut[1]}\wedge\ahist_2^\sharp\in\langof{\anaut[2]}}$
		\item $\anautp:=\bigcap\setcond{\alpha(\anobs[\aguarantee])}{\aguarantee\in\atypep}$
	\end{compactitem}

	First, assume $\langof{\anaut}\subset\langof{\anautp}$.
	We show that this implies~\eqref{eq:inference:history}.
	To that end, let $\ahist\in\typehistof{\athread}{\anadr}{\atype}$.
	By \Cref{thm:concrete-vs-abstract-induced-histories} we have $\alpha_\varphi(\ahist)\in\langof{\anaut[1]}$.
	Hence, $\alpha_\varphi(\ahist.\anevent)\in\langof{\anaut}$ by definition.
	So we get $\alpha_\varphi(\ahist.\anevent)\in\langof{\anautp}$ by assumption.
	Then, \Cref{thm:concrete-vs-abstract-induced-histories} yields the desired $\ahist.\anevent\in\typehistof{\athread}{\anadr}{\atypep}$.

	Now, assume implication~\eqref{eq:inference:history} holds.
	We show that $\langof{\anaut}\subseteq\langof{\anautp}$ follows.
	To that end, consider some $\ahist_1^\sharp\in\langof{\anaut}$.
	\Cref{thm:nonempty-history-concretisation} yields  $\ahist_1$ with $\ahist_1^\sharp=\alpha_\varphi(\ahist_1)$.
	By definition, $\ahist_1^\sharp$ is of the form $\ahist_1^\sharp=\ahist_2^\sharp.\anevent^\sharp$ for some $\ahist_2^\sharp\in\langof{\anaut[1]}$ and some $\anevent^\sharp\in\langof{\anaut[2]}$.
	Hence, there is $\ahist_2.\anevent$ with $\ahist_2^\sharp.\anevent^\sharp=\alpha_\varphi(\ahist_2.\anevent)$.
	Since $\ahist_2^\sharp\in\langof{\anaut[1]}$, we get $\ahist_2\in\typehistof{\athread}{\anadr}{\atype}$ by \Cref{thm:concrete-vs-abstract-induced-histories}.
	Then, the premise gives $\ahist_2.\anevent\in\typehistof{\athread}{\anadr}{\atype.\anevent}$.
	So, $\ahist_1\in\typehistof{\athread}{\anadr}{\atype.\anevent}$.
	Hence, \Cref{thm:concrete-vs-abstract-induced-histories} yields the desired $\ahist_1^\sharp\in\langof{\anautp}$.
\end{proof}
