# Supplementary material for: Pointer Life Cycle Types for Lock-Free Data Structures with Memory Reclamation
Source: arXiv:1910.11714 source file (2019-11-26)
Supplement: Supplementary file 2 [file reduction_proof_popl.tex]

%!TEX root = ../main.tex

\subsection{Full Proof of \CREF{thm:elision-computations-new}}
\label{proof:elision-computations}

\begin{proof}
	We proceed by induction over the structure of computations.

	\begin{description}[labelwidth=6mm,leftmargin=8mm,itemindent=0mm]
		\item[IB:]
			For $\tau=\epsilon$ choose $\sigma=\tau$.
			This satisfies the claim.

		\item[IH:]
			For every $\tau\in\allsemobs$ there is some $\sigma\in\freesemobs$ with the desired \Cref{proof:elision:premise:control,proof:elision:premise:valid-heap,proof:elision:premise:obsrel,proof:elision:premise:moreneq,proof:elision:premise:retired-new,proof:elision:premise:freed-not-retired,proof:elision:premise:fresh}.

		\item[IS:]
			Consider $\tau.\anact$.
			Let $\anact=(\athread,\acom,\anup)$.
			By induction there is $\sigma\in\freesemobs$ with:
			\begin{enumerate}[label=({P}\arabic*),leftmargin=1.3cm] % partopsep=1ex,parsep=1ex
				\item \label[property]{proof:elision:premise:control} $\controlof{\tau}=\controlof{\sigma}$
				\item \label[property]{proof:elision:premise:valid-heap} $\restrict{\heapcomput{\tau}}{\validof{\tau}}=\restrict{\heapcomput{\sigma}}{\validof{\sigma}}$
				\item \label[property]{proof:elision:premise:obsrel} $\forall\anadr\in\vadrof{\tau}.~\freeableof{\tau}{\anadr}\subseteq\freeableof{\sigma}{\anadr}$
				\item \label[property]{proof:elision:premise:moreneq} $\forall\anexp,\anexpp\in\pvars\cup\setcond{\psel{\anadr}}{\anadr\in\heapcomputof{\tau}{\validof{\tau}}}.~\heapcomputof{\tau}{\anexp}\neq\heapcomputof{\tau}{\anexpp}\implies\heapcomputof{\sigma}{\anexp}\neq\heapcomputof{\sigma}{\anexpp}$
				\item \label[property]{proof:elision:premise:retired-new} $\retiredof{\tau}\subseteq\retiredof{\sigma}$
				\item \label[property]{proof:elision:premise:freed-not-retired} $\freedof{\tau}\cap\retiredof{\tau}=\emptyset$
				\item \label[property]{proof:elision:premise:fresh} $\forall\anadr\in\freshof{\sigma}.~\freeableof{\tau}{\anadr}\subseteq\freeableof{\sigma}{\anadr}$
			\end{enumerate}
			\Cref{thm:valideq} yields:
			\begin{auxiliary}
				\label[aux]{proof:elision:aux:valid}
				\validof{\tau}=&\validof{\sigma}
			\end{auxiliary}
			We show that there is $\anactp$ with $\anactp=(\athread,\acom,\anupp)$ such that $\sigma.\anactp$ satisfies the desired properties:
			\begin{enumerate}[label=({G}\arabic*),leftmargin=1.3cm] % partopsep=1ex,parsep=1ex
				\item \label[property]{proof:elision:goal:control} $\controlof{\tau.\anact}=\controlof{\sigma.\anactp}$
				\item \label[property]{proof:elision:goal:valid-heap} $\restrict{\heapcomput{\tau.\anact}}{\validof{\tau.\anact}}=\restrict{\heapcomput{\sigma.\anactp}}{\validof{\sigma.\anactp}}$
				\item \label[property]{proof:elision:goal:obsrel} $\forall\anadr\in\vadrof{\tau.\anact}.~\freeableof{\tau.\anact}{\anadr}\subseteq\freeableof{\sigma.\anactp}{\anadr}$
				\item \label[property]{proof:elision:goal:moreneq} $\forall\anexp,\anexpp\in\pvars\cup\setcond{\psel{\anadr}}{\anadr\in\heapcomputof{\tau.\anact}{\validof{\tau.\anact}}}.~$\\$\heapcomputof{\tau.\anact}{\anexp}\neq\heapcomputof{\tau.\anact}{\anexpp}\implies\heapcomputof{\sigma.\anactp}{\anexp}\neq\heapcomputof{\sigma.\anactp}{\anexpp}$
				\item \label[property]{proof:elision:goal:retired-new} $\retiredof{\tau.\anact}\subseteq\retiredof{\sigma.\anactp}$
				\item \label[property]{proof:elision:goal:freed-not-retired} $\freedof{\tau.\anact}\cap\retiredof{\tau.\anact}=\emptyset$
				\item \label[property]{proof:elision:goal:fresh} $\forall\anadr\in\freshof{\sigma.\anact}.~\freeableof{\tau.\anact}{\anadr}\subseteq\freeableof{\sigma.\anact}{\anadr}$
			\end{enumerate}
			We do a case distinction over $\acom$.
			We will not comment on \Cref{proof:elision:goal:control} as it is guaranteed by the choice of $\anact$.
			We also only comment on $\historyof{\sigma.\anactp}\in\specof{\anobs}$ in the interesting cases according to \Cref{assumption:observers-accepting-state}, that is, when $\acom$ executes as a $\free$.
			\smallskip

			\begin{casedistinction}
		%=================================================================================================%
		%=================================================================================================%
		%=================================================================================================%
		%=================================================================================================%
				% \item[$\acom\equiv\invariantof{\_}$ or $\acom\equiv\ghostof{\_}$ or $\acom\equiv\cskip$ or $\acom\equiv\atomicbegin$ or $\acom\equiv\atomicend$]
				\item[$\acom\in\set{\invariantof{\bullet}\,,\, \atomicbegin,\, \atomicend}$]
				By definition, $\acom$ does not affect the computation, i.e., does not affect the memory nor the validity nor the history nor freedness nor freshness nor retiredness.
				This immediately gives \Cref{proof:elision:goal:valid-heap,proof:elision:goal:obsrel,proof:elision:goal:moreneq,proof:elision:goal:retired-new,proof:elision:goal:freed-not-retired,proof:elision:goal:fresh}.

		%=================================================================================================%
		%=================================================================================================%
		%=================================================================================================%
		%=================================================================================================%
				\item[$\acom\equiv\apvar=\apvarp$]
				The update is $\anup=[\apvar\mapsto\anadr]$ with $\heapcomputof{\tau}{\apvarp}=\anadr$.
				We choose $\anupp=[\apvar\mapsto\anadr']$ such that $\heapcomputof{\sigma}{\apvarp}=\anadr'$.
				Note that we have $\anadr=\anadr'$ if $\apvarp\in\validof{\tau}$.
				Otherwise, this equality may not hold.

				Since $\anact$/$\anactp$ does not change the retiredness we immediately get \Cref{proof:elision:goal:retired-new,proof:elision:goal:freed-not-retired,proof:elision:goal:fresh}.
				We show \Cref{proof:elision:goal:valid-heap,proof:elision:goal:obsrel,proof:elision:goal:moreneq}.

				%%%%%%%%%%%%%%%%%%%%%%%%%%%%%%%%%%%%%%%%%%%%%%%%%%%%%%%%%%%
				%%%%%%%%%%%%%%%%%%%%%%%%%%%%%%%%%%%%%%%%%%%%%%%%%%%%%%%%%%%
				\ad{\Cref{proof:elision:goal:valid-heap}}
				First consider the case where we have $\apvarp\in\validof{\tau}$.
				By \Cref{proof:elision:aux:valid} we also have $\apvarp\in\validof{\sigma}$.
				We get \[
					\restrict{\heapcomput{\tau.\anact}}{\validof{\tau.\anact}}
					=
					\restrict{\heapcomput{\tau}[\apvar\mapsto\anadr]}{\validof{\tau}\cup\set{\apvar}}
					=
					(\restrict{\heapcomput{\tau}}{\validof{\tau}})[\apvar\mapsto\anadr]
					\ .
				\]
				The second equality holds because $\heapcomputof{\tau}{\apvarp}=\anadr$.
				That is, we preserve $\dsel{\anadr}$ in $\restrict{\heapcomput{\tau}}{\validof{\tau}}$ and only need to update the mapping of $\apvar$.
				Similarly: \[
					\restrict{\heapcomput{\sigma.\anactp}}{\validof{\sigma.\anactp}}
					=
					\restrict{\heapcomput{\sigma}[\apvar\mapsto\anadr]}{\validof{\sigma}\cup\set{\apvar}}
					=
					(\restrict{\heapcomput{\sigma}}{\validof{\sigma}})[\apvar\mapsto\anadr]
				\]
				where $\anadr=\anadr'$ since $\apvarp\in\validof{\tau}$.
				We conclude $\restrict{\heapcomput{\sigma.\anactp}}{\validof{\sigma.\anactp}}=\restrict{\heapcomput{\tau.\anact}}{\validof{\tau.\anact}}$ by \Cref{proof:elision:premise:valid-heap}.

				Now consider the case $\apvarp\notin\validof{\tau}$.
				By \Cref{proof:elision:aux:valid} we have $\apvarp\notin\validof{\sigma}$.
				We get \[
					\restrict{\heapcomput{\tau.\anact}}{\validof{\tau.\anact}}
					=
					\restrict{\heapcomput{\tau}[\apvar\mapsto\anadr]}{\validof{\tau}\setminus\set{\apvar}}
					=
					\restrict{\heapcomput{\tau}}{\validof{\tau}\setminus\set{\apvar}}
					=
					\restrict{(\restrict{\heapcomput{\tau}}{\validof{\tau}})}{\validof{\tau}\setminus\set{\apvar}}
					\ .
				\]
				The second equality holds because the update does not survive the restriction to a set which does not to contain $\apvar$.
				The last equality is by definition of restrictions.
				Similarly, we get \[
					\restrict{\heapcomput{\sigma.\anactp}}{\validof{\sigma.\anactp}}
					=
					\restrict{\heapcomput{\sigma}[\apvar\mapsto\anadr']}{\validof{\sigma}\setminus\set{\apvar}}
					=
					\restrict{\heapcomput{\sigma}}{\validof{\sigma}\setminus\set{\apvar}}
					=
					\restrict{(\restrict{\heapcomput{\sigma}}{\validof{\sigma}})}{\validof{\sigma}\setminus\set{\apvar}}
					\ .
				\]
				Then we get $\restrict{\heapcomput{\tau}}{\validof{\tau}\setminus\set{\apvar}}=\restrict{\heapcomput{\sigma}}{\validof{\sigma}\setminus\set{\apvar}}$ by \Cref{proof:elision:premise:valid-heap} and \Cref{proof:elision:aux:valid}.
				This concludes the property.

				%%%%%%%%%%%%%%%%%%%%%%%%%%%%%%%%%%%%%%%%%%%%%%%%%%%%%%%%%%%
				%%%%%%%%%%%%%%%%%%%%%%%%%%%%%%%%%%%%%%%%%%%%%%%%%%%%%%%%%%%
				\ad{\Cref{proof:elision:goal:obsrel}}
				It suffices to show $\adrof{\restrict{\heapcomput{\tau.\anact}}{\validof{\tau.\anact}}}\subseteq\adrof{\restrict{\heapcomput{\tau}}{\validof{\tau}}}$ because of \Cref{proof:elision:premise:obsrel} and $\anact$/$\anactp$ not emitting an event.
				We have:
				\begin{align*}
					\adrof{\restrict{\heapcomput{\tau.\anact}}{\validof{\tau.\anact}}}
					=~&
					(\validof{\tau.\anact}\cap\adr)\cup\heapcomputof{\tau.\anact}{\validof{\tau.\anact}}
					\\\subseteq~&
					((\validof{\tau}\cup\set{\apvar})\cap\adr)\cup\heapcomputof{\tau.\anact}{\validof{\tau.\anact}}
					\\=~&
					(\validof{\tau}\cap\adr)\cup\heapcomputof{\tau.\anact}{\validof{\tau.\anact}}
				\end{align*}
				where the first equality is due to \Cref{thm:adrof-valid-heap-restriction}.
				It now remains to show that we have $\heapcomputof{\tau.\anact}{\validof{\tau.\anact}}\subseteq\heapcomputof{\tau}{\validof{\tau}}$.
				We do a case distinction.
				\begin{itemize}
					\item 
						If $\apvarp\notin\validof{\tau}$ we get:
						\begin{align*}
							\heapcomputof{\tau.\anact}{\validof{\tau.\anact}}
							=
							\heapcomputof{\tau.\anact}{\validof{\tau}\setminus\set{\apvar}}
							=
							\heapcomputof{\tau}{\validof{\tau}\setminus\set{\apvar}}
							\subseteq
							\heapcomputof{\tau}{\validof{\tau}}
							\ .
						\end{align*}

					\item
						If $\apvarp\in\validof{\tau}$ we get:
						\begin{align*}
							\heapcomputof{\tau.\anact}{\validof{\tau.\anact}}
							=~&
							\heapcomputof{\tau.\anact}{(\validof{\tau}\setminus\set{\apvar})\cup\set{\apvar}}
							=
							\heapcomputof{\tau}{\validof{\tau}\setminus\set{\apvar}}\cup\set{\anadr}
							\\\subseteq~&
							\heapcomputof{\tau}{\validof{\tau}}\cup\set{\anadr}
							=
							\heapcomputof{\tau}{\validof{\tau}}
						\end{align*}
						where the last equality holds because of $\heapcomputof{\tau}{\apvarp}=\anadr$ together with $\apvarp\in\validof{\tau}$ by assumption.
				\end{itemize}
				This concludes the property.

				%%%%%%%%%%%%%%%%%%%%%%%%%%%%%%%%%%%%%%%%%%%%%%%%%%%%%%%%%%%
				%%%%%%%%%%%%%%%%%%%%%%%%%%%%%%%%%%%%%%%%%%%%%%%%%%%%%%%%%%%
				\ad{\Cref{proof:elision:goal:moreneq}}
				Consider some $\anexp,\anexpp\in\pvars\cup\setcond{\psel{\anadr}}{\anadr\in\heapcomputof{\tau.\anact}{\validof{\tau.\anact}}}$ such that $\heapcomputof{\tau.\anact}{\anexp}\neq\heapcomputof{\tau.\anact}{\anexpp}$.
				We already showed $\heapcomputof{\tau.\anact}{\validof{\tau.\anact}}\subseteq\heapcomputof{\tau}{\validof{\tau}}$ for \Cref{proof:elision:goal:obsrel}.
				So $\anexp,\anexpp\in\pvars\cup\setcond{\psel{\anadr}}{\anadr\in\heapcomputof{\tau}{\validof{\tau}}}$.
				\begin{compactitem}
					\item
					If $\anexp\neq\apvar\neq\anexpp$, then we have $\heapcomputof{\tau}{\anexp}=\heapcomputof{\tau.\anact}{\anexp}\neq\heapcomputof{\tau.\anact}{\anexpp}=\heapcomputof{\tau}{\anexpp}$.
					From \Cref{proof:elision:premise:moreneq} we get $\heapcomputof{\sigma}{\anexp}\neq\heapcomputof{\sigma}{\anexpp}$.
					Thus $\heapcomputof{\sigma.\anactp}{\anexp}\neq\heapcomputof{\sigma.\anactp}{\anexpp}$ follows from $\heapcomputof{\sigma.\anactp}{\anexp}=\heapcomputof{\sigma}{\anexp}$ and $\heapcomputof{\sigma}{\anexpp}=\heapcomputof{\sigma.\anactp}{\anexpp}$.

					\item
					Consider wlog. $\anexp=\apvar$.
					So $\anexpp\neq\apvar$.
					We have $\heapcomputof{\tau}{\apvarp}=\heapcomputof{\tau.\anact}{\anexp}\neq\heapcomputof{\tau.\anact}{\anexpp}=\heapcomputof{\tau}{\anexpp}$.
					Hence, $\heapcomputof{\sigma}{\apvarp}\neq\heapcomputof{\sigma}{\anexpp}$ by \Cref{proof:elision:premise:moreneq}.
					We have $\heapcomputof{\sigma.\anactp}{\anexp}=\heapcomputof{\sigma}{\apvarp}$ and $\heapcomputof{\sigma.\anactp}{\anexpp}=\heapcomputof{\sigma}{\anexpp}$.
					So we get $\heapcomputof{\sigma.\anactp}{\anexp}\neq\heapcomputof{\sigma.\anactp}{\anexpp}$.
				\end{compactitem}
				The above case distinction is complete.
				This concludes the property.

		%=================================================================================================%
		%=================================================================================================%
		%=================================================================================================%
		%=================================================================================================%
				\item[$\acom\equiv\apvar=\psel{\apvarp}$]
				The update is $\anup=[\apvar\mapsto\anadrp]$ with $\heapcomputof{\tau}{\apvarp}=\anadr$ and $\heapcomputof{\tau}{\psel{\anadr}}=\anadrp$.
				By assumption, $\sigma$ is PRF.
				Hence, $\apvarp\in\validof{\sigma}$.
				So $\heapcomputof{\sigma}{\apvarp}=\heapcomputof{\tau}{\apvarp}=\anadr$.
				We choose $\anupp=[\apvar\mapsto\anadrp']$ with $\heapcomputof{\sigma}{\psel{\anadr}}$.

				Since $\anact$/$\anactp$ does not change the retiredness we immediately get \Cref{proof:elision:goal:retired-new,proof:elision:goal:freed-not-retired,proof:elision:goal:fresh}.
				We show \Cref{proof:elision:goal:valid-heap,proof:elision:goal:obsrel,proof:elision:goal:moreneq}.

				%%%%%%%%%%%%%%%%%%%%%%%%%%%%%%%%%%%%%%%%%%%%%%%%%%%%%%%%%%%
				%%%%%%%%%%%%%%%%%%%%%%%%%%%%%%%%%%%%%%%%%%%%%%%%%%%%%%%%%%%
				\ad{\Cref{proof:elision:goal:valid-heap}}
				First consider the case where we have $\psel{\anadr}\in\validof{\tau}$.
				By \Cref{proof:elision:aux:valid} this implies $\psel{\anadr}\in\validof{\sigma}$.
				That is, $\apvar$ is validated by the assignment.
				% Note that this gives $\apvarp\in\validof{\sigma}$ by \Cref{proof:gcplus:premise:valid}.
				We get \[
					\restrict{\heapcomput{\tau.\anact}}{\validof{\tau.\anact}}
					=
					\restrict{\heapcomput{\tau}[\apvar\mapsto\anadrp]}{\validof{\tau}\cup\set{\apvar}}
					=
					(\restrict{\heapcomput{\tau}}{\validof{\tau}})[\apvar\mapsto\anadrp]
					\ .
				\]
				The second equality holds because $\heapcomputof{\tau}{\psel{\anadr}}=\anadrp$.
				That is, we preserve $\dsel{\anadrp}$ in $\restrict{\heapcomput{\tau}}{\validof{\tau}}$ and only need to update the mapping of $\apvar$.
				Similarly, we get \[
					\restrict{\heapcomput{\sigma.\anactp}}{\validof{\sigma.\anactp}}
					=
					\restrict{\heapcomput{\sigma}[\apvar\mapsto\anadrp]}{\validof{\sigma}\cup\set{\apvar}}
					=
					(\restrict{\heapcomput{\sigma}}{\validof{\sigma}})[\apvar\mapsto\anadrp]
					\ .
				\]
				Then, $\restrict{\heapcomput{\sigma.\anactp}}{\validof{\sigma.\anactp}}=\restrict{\heapcomput{\tau.\anact}}{\validof{\tau.\anact}}$ follows from \Cref{proof:elision:premise:valid-heap}.

				Now consider the case $\psel{\anadr}\notin\validof{\tau}$.
				By \Cref{proof:elision:aux:valid} we have $\psel{\anadr}\notin\validof{\sigma}$.
				We get \[
					\restrict{\heapcomput{\tau.\anact}}{\validof{\tau.\anact}}
					=
					\restrict{\heapcomput{\tau}[\apvar\mapsto\anadrp]}{\validof{\tau}\setminus\set{\apvar}}
					=
					\restrict{\heapcomput{\tau}}{\validof{\tau}\setminus\set{\apvar}}
					=
					\restrict{(\restrict{\heapcomput{\tau}}{\validof{\tau}})}{\validof{\tau}\setminus\set{\apvar}}
					\ .
				\]
				The second equality holds because the update does not survive the restriction to a set which is guaranteed not to contain $\apvar$.
				Similarly, we have \[
					\restrict{\heapcomput{\sigma.\anactp}}{\validof{\sigma.\anactp}}
					=
					\restrict{\heapcomput{\sigma}[\apvar\mapsto\anadrp']}{\validof{\sigma}\setminus\set{\apvar}}
					=
					\restrict{\heapcomput{\sigma}}{\validof{\sigma}\setminus\set{\apvar}}
					=
					\restrict{(\restrict{\heapcomput{\sigma}}{\validof{\sigma}})}{\validof{\sigma}\setminus\set{\apvar}}
					\ .
				\]
				Then we get $\restrict{\heapcomput{\tau}}{\validof{\tau}\setminus\set{\apvar}}=\restrict{\heapcomput{\sigma}}{\validof{\sigma}\setminus\set{\apvar}}$ from \Cref{proof:elision:premise:valid-heap} and \Cref{proof:elision:aux:valid}.

				%%%%%%%%%%%%%%%%%%%%%%%%%%%%%%%%%%%%%%%%%%%%%%%%%%%%%%%%%%%
				%%%%%%%%%%%%%%%%%%%%%%%%%%%%%%%%%%%%%%%%%%%%%%%%%%%%%%%%%%%
				\ad{\Cref{proof:elision:goal:obsrel}}
				It suffices to show $\adrof{\restrict{\heapcomput{\tau.\anact}}{\validof{\tau.\anact}}}\subseteq\adrof{\restrict{\heapcomput{\tau}}{\validof{\tau}}}$ because of \Cref{proof:elision:premise:obsrel} and $\anact$/$\anactp$ not emitting an event.
				We have:
				\begin{align*}
					&
					\adrof{\restrict{\heapcomput{\tau.\anact}}{\validof{\tau.\anact}}}
					=
					(\validof{\tau.\anact}\cap\adr)\cup\heapcomputof{\tau.\anact}{\validof{\tau.\anact}}
					\\\subseteq~&
					((\validof{\tau}\cup\set{\apvar})\cap\adr)\cup\heapcomputof{\tau.\anact}{\validof{\tau.\anact}}
					=
					(\validof{\tau}\cap\adr)\cup\heapcomputof{\tau.\anact}{\validof{\tau.\anact}}
				\end{align*}
				where the first equality is due to \Cref{thm:adrof-valid-heap-restriction}.
				It now remains to show that we have $\heapcomputof{\tau.\anact}{\validof{\tau.\anact}}\subseteq\heapcomputof{\tau}{\validof{\tau}}$.
				We do a case distinction.
				\begin{itemize}
					\item
						If $\psel{\anadr}\notin\validof{\tau}$ we get:
						\begin{align*}
							\heapcomputof{\tau.\anact}{\validof{\tau.\anact}}
							=
							\heapcomputof{\tau.\anact}{\validof{\tau}\setminus\set{\apvar}}
							=
							\heapcomputof{\tau}{\validof{\tau}\setminus\set{\apvar}}
							\subseteq
							\heapcomputof{\tau}{\validof{\tau}}
						\end{align*}

					\item
						If $\psel{\anadr}\in\validof{\tau}$ we get:
						\begin{align*}
							\heapcomputof{\tau.\anact}{\validof{\tau.\anact}}
							=~&
							\heapcomputof{\tau.\anact}{(\validof{\tau}\setminus\set{\apvar})\cup\set{\apvar}}
							=
							\heapcomputof{\tau}{\validof{\tau}\setminus\set{\apvar}}\cup\set{\anadrp}
							\\\subseteq~&
							\heapcomputof{\tau}{\validof{\tau}}\cup\set{\anadrp}
							=
							\heapcomputof{\tau}{\validof{\tau}}
						\end{align*}
						where the last equality holds because of $\heapcomputof{\tau}{\psel{\anadr}}=\anadrp$ together with $\psel{\anadr}\in\validof{\tau}$ by assumption.
				\end{itemize}
				This concludes the property.

				%%%%%%%%%%%%%%%%%%%%%%%%%%%%%%%%%%%%%%%%%%%%%%%%%%%%%%%%%%%
				%%%%%%%%%%%%%%%%%%%%%%%%%%%%%%%%%%%%%%%%%%%%%%%%%%%%%%%%%%%
				\ad{\Cref{proof:elision:goal:moreneq}}
				Consider some $\anexp,\anexpp\in\pvars\cup\setcond{\psel{\anadr}}{\anadr\in\heapcomputof{\tau.\anact}{\validof{\tau.\anact}}}$ such that $\heapcomputof{\tau.\anact}{\anexp}\neq\heapcomputof{\tau.\anact}{\anexpp}$.
				We already showed $\heapcomputof{\tau.\anact}{\validof{\tau.\anact}}\subseteq\heapcomputof{\tau}{\validof{\tau}}$ for \Cref{proof:elision:goal:obsrel}.
				So $\anexp,\anexpp\in\pvars\cup\setcond{\psel{\anadr}}{\anadr\in\heapcomputof{\tau}{\validof{\tau}}}$.
				\begin{compactitem}
					\item
					If $\anexp\neq\apvar\neq\anexpp$, then we have $\heapcomputof{\tau}{\anexp}=\heapcomputof{\tau.\anact}{\anexp}\neq\heapcomputof{\tau.\anact}{\anexpp}=\heapcomputof{\tau}{\anexpp}$.
					From \Cref{proof:elision:premise:moreneq} we get $\heapcomputof{\sigma}{\anexp}\neq\heapcomputof{\sigma}{\anexpp}$.
					Thus $\heapcomputof{\sigma.\anactp}{\anexp}\neq\heapcomputof{\sigma.\anactp}{\anexpp}$ follows from $\heapcomputof{\sigma.\anactp}{\anexp}=\heapcomputof{\sigma}{\anexp}$ and $\heapcomputof{\sigma}{\anexpp}=\heapcomputof{\sigma.\anactp}{\anexpp}$.

					\item
					Consider wlog. $\anexp=\apvar$.
					So $\anexpp\neq\apvar$.
					We have $\heapcomputof{\tau}{\psel{\anadr}}=\heapcomputof{\tau.\anact}{\anexp}\neq\heapcomputof{\tau.\anact}{\anexpp}=\heapcomputof{\tau}{\anexpp}$.
					Hence, $\heapcomputof{\sigma}{\psel{\anadr}}\neq\heapcomputof{\sigma}{\anexpp}$ by \Cref{proof:elision:premise:moreneq}.
					We have $\heapcomputof{\sigma.\anactp}{\anexp}=\heapcomputof{\sigma}{\psel{\anadr}}$ and $\heapcomputof{\sigma.\anactp}{\anexpp}=\heapcomputof{\sigma}{\anexpp}$.
					So we get $\heapcomputof{\sigma.\anactp}{\anexp}\neq\heapcomputof{\sigma.\anactp}{\anexpp}$.
				\end{compactitem}
				The above case distinction is complete.
				This concludes the property.

		%=================================================================================================%
		%=================================================================================================%
		%=================================================================================================%
		%=================================================================================================%
				\item[$\acom\equiv\psel{\apvar}=\apvarp$]
				This case is analogous to the previous one.

		%=================================================================================================%
		%=================================================================================================%
		%=================================================================================================%
		%=================================================================================================%
				\item[$\acom\equiv\advar=\opof{\advar_1,\ldots, \advar_n}$]
				The update is $\anup=[\advar\mapsto\advalue]$ with $\advalue=\opof{\heapcomputof{\tau}{\advar_1},\dots,\heapcomputof{\tau}{\advar_n}}$.
				By definition, we have $\advar_1,\dots,\advar_n\in\domof{\restrict{\heapcomput{\tau}}{\validof{\tau}}}$.
				So \Cref{proof:elision:premise:valid-heap} gives $\advalue=\opof{\heapcomputof{\sigma}{\advar_1},\dots,\heapcomputof{\sigma}{\advar_n}}$.
				Hence, we choose $\anupp=\anup$.
				That is, the same update is performed, $\anup=\anupp$.
				We immediately get \Cref{proof:elision:goal:valid-heap,proof:elision:goal:obsrel,proof:elision:goal:moreneq,proof:elision:goal:retired-new,proof:elision:goal:freed-not-retired,proof:elision:goal:fresh}.

		%=================================================================================================%
		%=================================================================================================%
		%=================================================================================================%
		%=================================================================================================%
				\item[$\acom\equiv\advar=\dsel{\apvarp}$]
				The update is $\anup=[\advar\mapsto\advalue]$ with $\heapcomputof{\tau}{\apvarp}=\anadr$ and $\heapcomputof{\tau}{\dsel{\anadr}}=\advalue$.
				By assumption, $\sigma$ is PRF.
				Hence, $\apvarp\in\validof{\sigma}$.
				That is, $\heapcomputof{\sigma}{\apvarp}=\anadr$ and $\heapcomputof{\sigma}{\dsel{\anadr}}=\advalue$ by \Cref{proof:elision:premise:valid-heap}.
				We choose $\anupp=\anup$ and immediately get \Cref{proof:elision:goal:valid-heap,proof:elision:goal:obsrel,proof:elision:goal:moreneq,proof:elision:goal:retired-new,proof:elision:goal:freed-not-retired,proof:elision:goal:fresh}.

		%=================================================================================================%
		%=================================================================================================%
		%=================================================================================================%
		%=================================================================================================%
				\item[$\acom\equiv\dsel{\apvar}=\advarp$]
				The update is $\anup=[\dsel{\anadr}\mapsto\advalue]$ with $\heapcomputof{\tau}{\apvar}=\anadr$ and $\heapcomputof{\tau}{\advarp}=\advalue$.
				By assumption, $\sigma$ is PRF.
				Hence, $\apvar\in\validof{\sigma}$.
				That is, $\heapcomputof{\sigma}{\apvar}=\anadr$ and $\heapcomputof{\sigma}{\advarp}=\advalue$ by \Cref{proof:elision:premise:valid-heap}.
				We choose $\anupp=\anup$ and immediately get \Cref{proof:elision:goal:valid-heap,proof:elision:goal:obsrel,proof:elision:goal:moreneq,proof:elision:goal:retired-new,proof:elision:goal:freed-not-retired,proof:elision:goal:fresh}.

		%=================================================================================================%
		%=================================================================================================%
		%=================================================================================================%
		%=================================================================================================%
				\item[$\acom\equiv\assumeof{\apvar=\apvarp}$]
				By assumption, $\sigma$ is PRF.
				So $\apvar,\apvarp\in\validof{\sigma}$ and thus $\heapcomputof{\sigma}{\apvar}=\heapcomputof{\tau}{\apvar}=\heapcomputof{\tau}{\apvarp}=\heapcomputof{\sigma}{\apvarp}$.
				Then, $\anactp=\anact$ is indeed enabled after $\sigma$.
				The updates are $\anup=\anupp=\emptyset$.

				Since $\anact$/$\anactp$ does not change the retiredness and freshness we immediately get \Cref{proof:elision:goal:retired-new,proof:elision:goal:freed-not-retired,proof:elision:goal:fresh}.
				We show \Cref{proof:elision:goal:valid-heap,proof:elision:goal:obsrel,proof:elision:goal:moreneq}.
				To do so, we first show the following auxiliary statements:
				\begin{auxiliary}
					\heapcomputof{\tau.\anact}{\validof{\tau.\anact}}&=\heapcomputof{\tau}{\validof{\tau}}
					\label[aux]{proof:elision:asserteq:valid-heap-tau}
					\\
					\heapcomputof{\sigma.\anactp}{\validof{\sigma.\anactp}}&=\heapcomputof{\sigma}{\validof{\sigma}}
					\label[aux]{proof:elision:asserteq:valid-heap-sigma}
					\\
					\validof{\tau.\anact}&=\validof{\sigma.\anactp}
					\label[aux]{proof:elision:asserteq:valid-act}
				\end{auxiliary}

				%%%%%%%%%%%%%%%%%%%%%%%%%%%%%%%%%%%%%%%%%%%%%%%%%%%%%%%%%%%
				%%%%%%%%%%%%%%%%%%%%%%%%%%%%%%%%%%%%%%%%%%%%%%%%%%%%%%%%%%%
				\ad{\Cref{proof:elision:asserteq:valid-heap-tau}}
				It suffices to show $\heapcomputof{\tau}{\validof{\tau.\anact}}=\heapcomputof{\tau}{\validof{\tau}}$ since $\heapcomput{\tau.\anact}=\heapcomput{\tau}$.
				If $\validof{\tau.\anact}=\validof{\tau}$, then claim follows immediately.
				So assume $\validof{\tau.\anact}\neq\validof{\tau}$.
				By definition, we get $\validof{\tau.\anact}=\validof{\tau}\cup\set{\apvar,\apvarp}$ and $\set{\apvar,\apvarp}\cap\validof{\tau}\neq\emptyset$.
				Wlog. let $\apvar\in\validof{\tau}$.
				So $\heapcomputof{\tau}{\apvar}\in\heapcomputof{\tau}{\validof{\tau}}$.
				And because $\heapcomputof{\tau}{\apvar}=\heapcomputof{\tau}{\apvarp}$ we also get $\heapcomputof{\tau}{\apvarp}\in\heapcomputof{\tau}{\validof{\tau}}$.
				Hence, we conclude by: \[\heapcomputof{\tau}{\validof{\tau.\anact}}=\heapcomputof{\tau}{\validof{\tau}\cup\set{\apvar,\apvarp}}=\heapcomputof{\tau}{\validof{\tau}} \ .\]

				%%%%%%%%%%%%%%%%%%%%%%%%%%%%%%%%%%%%%%%%%%%%%%%%%%%%%%%%%%%
				%%%%%%%%%%%%%%%%%%%%%%%%%%%%%%%%%%%%%%%%%%%%%%%%%%%%%%%%%%%
				\ad{\Cref{proof:elision:asserteq:valid-heap-sigma}}
				Analogous to \Cref{proof:elision:asserteq:valid-heap-tau}.

				%%%%%%%%%%%%%%%%%%%%%%%%%%%%%%%%%%%%%%%%%%%%%%%%%%%%%%%%%%%
				%%%%%%%%%%%%%%%%%%%%%%%%%%%%%%%%%%%%%%%%%%%%%%%%%%%%%%%%%%%
				\ad{\Cref{proof:elision:asserteq:valid-act}}
				There are two cases.
				\begin{compactitem}
					\item
					Consider $\set{\apvar,\apvarp}\cap\validof{\tau}=\emptyset$
					Then, \Cref{proof:elision:aux:valid} gives $\set{\apvar,\apvarp}\cap\validof{\sigma}=\emptyset$.
					By definition, this gives $\validof{\tau.\anact}=\validof{\tau}$ and $\validof{\sigma.\anactp}=\validof{\sigma}$.
					Hence, the claim follows from \Cref{proof:elision:aux:valid}.

					\item
					Consider $\set{\apvar,\apvarp}\cap\validof{\tau}\neq\emptyset$.
					Wlog. $\apvar\in\validof{\tau}$.
					By \Cref{proof:elision:aux:valid} we have $\apvar\in\validof{\sigma}$.
					And by definition, we get $\validof{\tau.\anact}=\validof{\tau}\cup\set{\apvar,\apvarp}$ and $\validof{\sigma.\anactp}=\validof{\sigma}\cup\set{\apvar,\apvarp}$.
					Again, we conclude by \Cref{proof:elision:aux:valid}.
				\end{compactitem}
				The above case distinction is complete and thus proves the claim.

				%%%%%%%%%%%%%%%%%%%%%%%%%%%%%%%%%%%%%%%%%%%%%%%%%%%%%%%%%%%
				%%%%%%%%%%%%%%%%%%%%%%%%%%%%%%%%%%%%%%%%%%%%%%%%%%%%%%%%%%%
				\ad{\Cref{proof:elision:goal:valid-heap}}
				We consider two cases.
				First, assume $\set{\apvar,\apvarp}\cap\validof{\tau}=\emptyset$.
				Then, we have $\validof{\tau.\anact}=\validof{\tau}$.
				So \Cref{proof:elision:asserteq:valid-act} together with \Cref{proof:elision:aux:valid} gives $\validof{\sigma.\anactp}=\validof{\sigma}$.
				Hence, we can conclude using $\heapcomput{\tau.\anact}=\heapcomput{\tau}$ and $\heapcomput{\sigma.\anactp}=\heapcomput{\sigma}$: \[\restrict{\heapcomput{\tau.\anact}}{\validof{\tau.\anact}}=\restrict{\heapcomput{\tau}}{\validof{\tau}}=\restrict{\heapcomput{\sigma}}{\validof{\sigma}}=\restrict{\heapcomput{\sigma.\anactp}}{\validof{\sigma.\anactp}}\] where the second equality holds by \Cref{proof:elision:premise:valid-heap}.

				Second, assume $\set{\apvar,\apvarp}\cap\validof{\tau}\neq\emptyset$.
				Then, $\validof{\tau.\anact}=\validof{\tau}\cup\set{\apvar,\apvarp}$.
				So \Cref{proof:elision:asserteq:valid-act} together with \Cref{proof:elision:aux:valid} gives $\validof{\sigma.\anactp}=\validof{\sigma}\cup\set{\apvar,\apvarp}$.
				Using \Cref{proof:elision:asserteq:valid-heap-tau,proof:elision:asserteq:valid-heap-sigma} and \Cref{proof:elision:premise:valid-heap} we now get:
				\begin{align*}
					&\domof{\restrict{\heapcomput{\tau.\anact}}{\validof{\tau.\anact}}}
					\\=~&
					\validof{\tau.\anact}\cup\dvars\cup\setcond{\dsel{\anadrpp}}{\anadrpp\in\heapcomputof{\tau.\anact}{\validof{\tau.\anact}}}
					\\=~&
					\validof{\tau}\cup\set{\apvar,\apvarp}\cup\dvars\cup\setcond{\dsel{\anadrpp}}{\anadrpp\in\heapcomputof{\tau}{\validof{\tau}}}
					\\=~&
					\domof{\restrict{\heapcomput{\tau}}{\validof{\tau}}}\cup\set{\apvar,\apvarp}
					\\=~&
					\domof{\restrict{\heapcomput{\sigma}}{\validof{\sigma}}}\cup\set{\apvar,\apvarp}
					\\=~&
					\validof{\sigma}\cup\set{\apvar,\apvarp}\cup\dvars\cup\setcond{\dsel{\anadrpp}}{\anadrpp\in\heapcomputof{\sigma}{\validof{\sigma}}}
					\\=~&
					\validof{\sigma.\anactp}\cup\dvars\cup\setcond{\dsel{\anadrpp}}{\anadrpp\in\heapcomputof{\sigma.\anactp}{\validof{\sigma.\anactp}}}
					\\=~&
					\domof{\restrict{\heapcomput{\sigma.\anactp}}{\validof{\sigma.\anactp}}}
				\end{align*}
				By \Cref{proof:elision:premise:valid-heap} together with $\heapcomput{\tau.\anact}=\heapcomput{\tau}$ and $\heapcomput{\sigma.\anactp}=\heapcomput{\sigma}$ it remains to show \[\heapcomputof{\tau.\anact}{\apvar}=\heapcomputof{\sigma.\anactp}{\apvar} \qquad\text{and}\qquad \heapcomputof{\tau.\anact}{\apvarp}=\heapcomputof{\sigma.\anactp}{\apvarp}\ .\]
				Wlog. $\apvar\in\validof{\tau}$.
				Then, $\heapcomputof{\tau}{\apvar}=\heapcomputof{\sigma}{\apvar}$.
				Hence, $\heapcomputof{\tau.\anact}{\apvar}=\heapcomputof{\sigma.\anactp}{\apvar}$.
				And the assertion in $\acom$ requires $\apvar$ and $\apvarp$ to have the same valuation, ${\heapcomputof{\tau.\anact}{\apvarp}=\heapcomputof{\sigma.\anactp}{\apvarp}}$.
				This concludes the claim.

				%%%%%%%%%%%%%%%%%%%%%%%%%%%%%%%%%%%%%%%%%%%%%%%%%%%%%%%%%%%
				%%%%%%%%%%%%%%%%%%%%%%%%%%%%%%%%%%%%%%%%%%%%%%%%%%%%%%%%%%%
				\ad{\Cref{proof:elision:goal:obsrel}}
				We have $\freeableof{\tau.\anact}{\anadrpp}=\freeableof{\tau}{\anadrpp}$ and $\freeableof{\sigma.\anactp}{\anadrpp}=\freeableof{\sigma}{\anadrpp}$ for all $\anadrpp\in\adr$ since $\anact$/$\anactp$ does not emit an event.
				Using \Cref{thm:adrof-valid-heap-restriction} and \Cref{proof:elision:asserteq:valid-heap-tau} we get:
				\begin{align*}
					&
					\adrof{\restrict{\heapcomput{\tau.\anact}}{\validof{\tau.\anact}}}
					=
					(\validof{\tau.\anact}\cap\adr)\cup\heapcomputof{\tau.\anact}{\validof{\tau.\anact}}
					\\\subseteq~&
					((\validof{\tau}\cup{\apvar,\apvarp})\cap\adr)\cup\heapcomputof{\tau}{\validof{\tau}}
					\\=~&
					(\validof{\tau}\cap\adr)\cup\heapcomputof{\tau}{\validof{\tau}}
					=
					\adrof{\restrict{\heapcomput{\tau}}{\validof{\tau}}}
					\ .
				\end{align*}
				This concludes the claim by \Cref{proof:elision:premise:obsrel}.

				%%%%%%%%%%%%%%%%%%%%%%%%%%%%%%%%%%%%%%%%%%%%%%%%%%%%%%%%%%%
				%%%%%%%%%%%%%%%%%%%%%%%%%%%%%%%%%%%%%%%%%%%%%%%%%%%%%%%%%%%
				\ad{\Cref{proof:elision:goal:moreneq}}
				Consider some $\anexp,\anexpp\in\pvars\cup\setcond{\psel{\anadr}}{\anadr\in\heapcomputof{\tau.\anact}{\validof{\tau.\anact}}}$ such that $\heapcomputof{\tau.\anact}{\anexp}\neq\heapcomputof{\tau.\anact}{\anexpp}$.
				Since $\anup=\emptyset$, we get $\heapcomputof{\tau}{\anexp}\neq\heapcomputof{\tau}{\anexpp}$.
				Moreover, by \Cref{proof:elision:asserteq:valid-heap-tau}, we have $\anexp,\anexpp\in\pvars\cup\setcond{\psel{\anadr}}{\anadr\in\heapcomputof{\tau.\anact}{\validof{\tau.\anact}}}$.
				Hence, $\heapcomputof{\sigma}{\anexp}\neq\heapcomputof{\sigma}{\anexpp}$.
				As consequence, we get $\heapcomputof{\sigma.\anactp}{\anexp}\neq\heapcomputof{\sigma.\anactp}{\anexpp}$ since $\anupp=\emptyset$.
				This concludes the property.

		%=================================================================================================%
		%=================================================================================================%
		%=================================================================================================%
		%=================================================================================================%
				\item[$\acom\equiv\assumeof{\apvar\neq\apvarp}$]
				We have $\heapcomputof{\tau}{\apvar}\neq\heapcomputof{\tau}{\apvarp}$.
				The update is $\anup=\emptyset$.
				We choose $\anupp=\emptyset$.
				By \Cref{proof:elision:premise:moreneq}, we get $\heapcomputof{\sigma}{\apvar}\neq\heapcomputof{\sigma}{\apvarp}$.
				So $\anactp$ is indeed enabled after $\sigma$.
				We immediately get \Cref{proof:elision:goal:valid-heap,proof:elision:goal:obsrel,proof:elision:goal:moreneq,proof:elision:goal:retired-new,proof:elision:goal:freed-not-retired,proof:elision:goal:fresh}.

		%=================================================================================================%
		%=================================================================================================%
		%=================================================================================================%
		%=================================================================================================%
				\item[$\acom\equiv\assumeof{\predof{\vecof{\advar}}}$]
				We have $\anup=\anupp=\emptyset$ by definition.
				Let $\vecof{\advar}=\advar_1,\dots,\advar_n$.
				Then, $\advar_1,\dots,\advar_n\in\domof{\restrict{\heapcomput{\tau}}{\validof{\tau}}}$ by definition.
				So $\heapcomputof{\tau}{\advar}=\heapcomputof{\sigma}{\advar}$ and $\heapcomputof{\tau}{\advarp}=\heapcomputof{\sigma}{\advarp}$ \Cref{proof:elision:premise:valid-heap}.
				That is, $\anactp$ is enabled after $\sigma$ indeed.
				We immediately get \Cref{proof:elision:goal:valid-heap,proof:elision:goal:obsrel,proof:elision:goal:moreneq,proof:elision:goal:retired-new,proof:elision:goal:freed-not-retired,proof:elision:goal:fresh}.

		%=================================================================================================%
		%=================================================================================================%
		%=================================================================================================%
		%=================================================================================================%
				\item[$\acom\equiv\enterof{\afuncof{\vecof{\apvar},\vecof{\advar}}}$]
				We have $\anup=\anupp=\emptyset$.
				Since $\anact$/$\anactp$ does not have an effect on the memory, and validity, we immediately get \Cref{proof:elision:goal:valid-heap,proof:elision:goal:moreneq}.
				It remains to show \Cref{proof:elision:goal:obsrel,proof:elision:goal:retired-new,proof:elision:goal:freed-not-retired,proof:elision:goal:fresh}.

				%%%%%%%%%%%%%%%%%%%%%%%%%%%%%%%%%%%%%%%%%%%%%%%%%%%%%%%%%%%
				%%%%%%%%%%%%%%%%%%%%%%%%%%%%%%%%%%%%%%%%%%%%%%%%%%%%%%%%%%%
				\ad{\Cref{proof:elision:goal:obsrel}}
				Let $\vecof{\anadr}=\heapcomputof{\sigma}{\vecof{\apvar}}$, $\vecof{\anadrp}=\heapcomputof{\tau}{\vecof{\apvar}}$, $\vecof{\advalue}=\heapcomputof{\sigma}{\vecof{\advar}}$.
				By \Cref{proof:elision:premise:valid-heap}, we have $\heapcomputof{\tau}{\vecof{\advar}}=\vecof{\advalue}$.
				Let $\anadrpp\in\vadrof{\tau.\anact}=\vadrof{\tau}$.
				If $\anadr_i=\anadrpp$, then $\apvar_i\in\validof{\sigma}$ by \Cref{thm:invalidpointers-adr}.
				By \Cref{proof:elision:premise:valid-heap} this means $\anadrp_i=\anadrpp$.
				Altogether, we have: $\anadr_i=\anadrpp$ implies $\anadrp_i=\anadrpp$.
				Now, let $\ahist=\historyof{\tau}$ and let $\ahistp=\historyof{\sigma}$.
				Note that $\historyof{\tau.\anact}=\ahist.\evt{\afunc}{\athread,\vecof{\anadrp},\vecof{\advalue}}$ and $\historyof{\sigma.\anactp}=\ahistp.\evt{\afunc}{\athread,\vecof{\anadr},\vecof{\advalue}}$.
				Since $\sigma.\anact$ is PRF, we get \[\freeableof{\ahistp.\evt{\afunc}{\athread,\vecof{\anadrp},\vecof{\advalue}}}{\anadrpp}\subseteq\freeableof{\ahistp.\evt{\afunc}{\athread,\vecof{\anadr},\vecof{\advalue}}}{\anadrpp}\ .\]
				It remains to show \[\freeableof{\ahist.\evt{\afunc}{\athread,\vecof{\anadrp},\vecof{\advalue}}}{\anadrpp}\subseteq\freeableof{\ahistp.\evt{\afunc}{\athread,\vecof{\anadrp},\vecof{\advalue}}}{\anadrpp}\ .\]
				To see this, consider $\ahistpp\in\freeableof{\ahist.\evt{\afunc}{\athread,\vecof{\anadrp},\vecof{\advalue}}}{\anadrpp}$.
				We get $\ahistpp.\evt{\afunc}{\athread,\vecof{\anadrp},\vecof{\advalue}}\in\freeableof{\ahist}{\anadrpp}$ from \Cref{thm:move-event-from-freeable}.
				So by \Cref{proof:elision:premise:obsrel} we have $\ahistpp.\evt{\afunc}{\athread,\vecof{\anadrp},\vecof{\advalue}}\in\freeableof{\ahistp}{\anadrpp}$.
				Again by \Cref{thm:move-event-from-freeable}, we get $\ahistpp\in\freeableof{\ahistp.\evt{\afunc}{\athread,\vecof{\anadrp},\vecof{\advalue}}}{\anadrpp}$.
				This concludes the claim.

				%%%%%%%%%%%%%%%%%%%%%%%%%%%%%%%%%%%%%%%%%%%%%%%%%%%%%%%%%%%
				%%%%%%%%%%%%%%%%%%%%%%%%%%%%%%%%%%%%%%%%%%%%%%%%%%%%%%%%%%%
				\ad{\Cref{proof:elision:goal:retired-new}}
				If $\afuncof{\vecof{\apvar},\vecof{\advar}}\not\equiv\retireof{\apvar}$, then the claim follows from \Cref{proof:elision:premise:retired-new}.
				So consider $\afuncof{\vecof{\apvar},\vecof{\advar}}\equiv\retireof{\apvar}$.
				Since $\freesem$ is PRF, we know that $\sigma.\anactp$ is pointer race free.
				Hence, $\apvar\in\validof{\sigma}$.
				By \Cref{proof:elision:aux:valid} we have $\apvar\in\validof{\tau}$.
				By \Cref{proof:elision:premise:valid-heap} we have $\heapcomputof{\tau}{\apvar}=\heapcomputof{\sigma}{\apvar}=\anadr$.
				So by definition, we have $\retiredof{\tau.\anact}=\retiredof{\tau}\cup\set{\anadr}$ and similarly $\retiredof{\sigma.\anactp}=\retiredof{\sigma}\cup\set{\anadr}$.
				Hence, the claim follows from \Cref{proof:elision:premise:valid-heap}.

				%%%%%%%%%%%%%%%%%%%%%%%%%%%%%%%%%%%%%%%%%%%%%%%%%%%%%%%%%%%
				%%%%%%%%%%%%%%%%%%%%%%%%%%%%%%%%%%%%%%%%%%%%%%%%%%%%%%%%%%%
				\ad{\Cref{proof:elision:goal:freed-not-retired}}
				If $\afuncof{\vecof{\apvar},\vecof{\advar}}\not\equiv\retireof{\apvar}$, then the claim follows from \Cref{proof:elision:premise:retired-new}.
				So consider $\afuncof{\vecof{\apvar},\vecof{\advar}}\equiv\retireof{\apvar}$.
				As for \Cref{proof:elision:goal:retired-new} above, we conclude $\apvar\in\validof{\sigma}$.
				Then, the contrapositive of \Cref{thm:pointers-to-freed-are-invalid} yields $\heapcomputof{\tau}{\apvar}\notin\freedof{\tau}$.
				This means $\heapcomputof{\tau}{\apvar}\notin\freedof{\tau.\anact}$ by definition.
				Hence, the claim follows from \Cref{proof:elision:premise:freed-not-retired}

				%%%%%%%%%%%%%%%%%%%%%%%%%%%%%%%%%%%%%%%%%%%%%%%%%%%%%%%%%%%
				%%%%%%%%%%%%%%%%%%%%%%%%%%%%%%%%%%%%%%%%%%%%%%%%%%%%%%%%%%%
				\ad{\Cref{proof:elision:goal:fresh}}
				Let $\vecof{\anadr}=\heapcomputof{\sigma}{\vecof{\apvar}}$, $\vecof{\anadrp}=\heapcomputof{\tau}{\vecof{\apvar}}$, $\vecof{\advalue}=\heapcomputof{\sigma}{\vecof{\advar}}$.
				By \Cref{proof:elision:premise:valid-heap}, we have $\heapcomputof{\tau}{\vecof{\advar}}=\vecof{\advalue}$.
				Let $\anadrpp\in\freshof{\sigma.\anact}$.
				Note that $\freshof{\sigma.\anact}=\freshof{\sigma}$.
				Let $\ahist=\historyof{\tau}$ and let $\ahistp=\historyof{\sigma}$.
				Note that $\historyof{\tau.\anact}=\ahist.\evt{\afunc}{\athread,\vecof{\anadrp},\vecof{\advalue}}$ and $\historyof{\sigma.\anactp}=\ahistp.\evt{\afunc}{\athread,\vecof{\anadr},\vecof{\advalue}}$.
				Since $\sigma.\anact$ is PRF, we get \[\freeableof{\ahistp.\evt{\afunc}{\athread,\vecof{\anadrp},\vecof{\advalue}}}{\anadrpp}\subseteq\freeableof{\ahistp.\evt{\afunc}{\athread,\vecof{\anadr},\vecof{\advalue}}}{\anadrpp}\ .\]
				It remains to show \[\freeableof{\ahist.\evt{\afunc}{\athread,\vecof{\anadrp},\vecof{\advalue}}}{\anadrpp}\subseteq\freeableof{\ahistp.\evt{\afunc}{\athread,\vecof{\anadrp},\vecof{\advalue}}}{\anadrpp}\ .\]
				Similarly to the reasoning for \Cref{proof:elision:goal:obsrel}, this follows from \Cref{thm:move-event-from-freeable} and \Cref{proof:elision:premise:fresh}.

		%=================================================================================================%
		%=================================================================================================%
		%=================================================================================================%
		%=================================================================================================%
				\item[$\acom\equiv\exitof{\afunc}$]
				The updates are $\anup=\anupp=\emptyset$.
				Since $\anact$/$\anactp$ does not have an effect on the memory, and validity, we immediately get \Cref{proof:elision:goal:valid-heap,proof:elision:goal:moreneq,proof:elision:goal:retired-new,proof:elision:goal:freed-not-retired}.
				For \Cref{proof:elision:goal:obsrel} note that $\historyof{\tau.\anact}=\historyof{\tau}.\evt{\exitof{\afunc}}{\athread}$ and $\historyof{\sigma.\anactp}=\historyof{\sigma}.\evt{\exitof{\afunc}}{\athread}$.
				That is, both $\anact$ and $\anactp$ emit the same event.
				Then the claim follows from \Cref{proof:elision:premise:obsrel} and \Cref{thm:move-event-from-freeable}.
				Similarly, for \Cref{proof:elision:goal:fresh}.

		%=================================================================================================%
		%=================================================================================================%
		%=================================================================================================%
		%=================================================================================================%
				\item[$\acom\equiv\freeof{\anadr}$ and $\historyof{\sigma}.\freeof{\anadr}\in\specof{\anobs}$]
				The updates are $\anup=\anupp=\emptyset$.
				By the case assumption $\anactp$ is indeed enabled after $\sigma$.
				We show \Cref{proof:elision:goal:valid-heap,proof:elision:goal:obsrel,proof:elision:goal:moreneq,proof:elision:goal:retired-new,proof:elision:goal:freed-not-retired,proof:elision:goal:fresh}.

				%%%%%%%%%%%%%%%%%%%%%%%%%%%%%%%%%%%%%%%%%%%%%%%%%%%%%%%%%%%
				%%%%%%%%%%%%%%%%%%%%%%%%%%%%%%%%%%%%%%%%%%%%%%%%%%%%%%%%%%%
				\ad{\Cref{proof:elision:goal:valid-heap}}
				First, note that $\validof{\tau.\anact}=\validof{\sigma.\anactp}$.
				To see this, consider $\apexp\in\validof{\tau.\anact}$.
				By definition, this means $\apexp\in\validof{\tau}$, $\apexp\not\equiv\psel{\anadr}$, and $\heapcomputof{\tau}{\apexp}\neq\anadr$.
				From \Cref{proof:elision:aux:valid} we get $\apexp\in\validof{\sigma}$.
				From \Cref{proof:elision:premise:valid-heap} we get $\heapcomputof{\sigma}{\apexp}=\heapcomputof{\tau}{\apexp}\neq\anadr$.
				Hence, $\apexp\in\validof{\sigma.\anactp}$ must hold by definition.
				This establishes $\validof{\tau.\anact}\subseteq\validof{\sigma.\anactp}$.
				The reverse inclusion follows analogously.
				So we have $\validof{\tau.\anact}=\validof{\sigma.\anactp}$ indeed.
				Second, note that we have $\validof{\tau.\anact}\subseteq\validof{\tau}$ and $\validof{\sigma.\anactp}\subseteq\validof{\sigma}$.
				Third, note that $\heapcomput{\tau}=\heapcomput{\tau.\anact}$ and $\heapcomput{\sigma}=\heapcomput{\sigma.\anactp}$.
				Then, we conclude as follows:
				\begin{align*}
					\restrict{\heapcomput{\tau.\anact}}{\validof{\tau.\anact}}
					&=
					\restrict{\heapcomput{\tau}}{\validof{\tau.\anact}}
					=
					\restrict{(\restrict{\heapcomput{\tau}}{\validof{\tau}})}{\validof{\tau.\anact}}
					\\&=
					\restrict{(\restrict{\heapcomput{\sigma}}{\validof{\sigma}})}{\validof{\tau.\anact}}
					=
					\restrict{(\restrict{\heapcomput{\sigma}}{\validof{\sigma}})}{\validof{\sigma.\anactp}}
					\\&=
					\restrict{\heapcomput{\sigma}}{\validof{\sigma.\anactp}}
					=
					\restrict{\heapcomput{\sigma.\anactp}}{\validof{\sigma.\anactp}}
				\end{align*}
				where the third equality is due to \Cref{proof:elision:premise:valid-heap}.

				%%%%%%%%%%%%%%%%%%%%%%%%%%%%%%%%%%%%%%%%%%%%%%%%%%%%%%%%%%%
				%%%%%%%%%%%%%%%%%%%%%%%%%%%%%%%%%%%%%%%%%%%%%%%%%%%%%%%%%%%
				\ad{\Cref{proof:elision:goal:obsrel}}
				Let $\anadrp\in\vadrof{\tau.\anact}$.
				We have $\anadrp\in\vadrof{\tau}$ by definition.
				Let $\ahist\in\freeableof{\tau.\anact}{\anadrp}$.
				Note that we have $\historyof{\tau.\anact}=\historyof{\tau}.\freeof{\anadr}$.
				So, $\freeof{\anadr}.\ahist\in\freeableof{\tau}{\anadrp}$ by \Cref{thm:move-event-from-freeable}.
				By \Cref{proof:elision:premise:obsrel} we get $\freeof{\anadr}.\ahist\in\freeableof{\sigma}{\anadrp}$.
				Again by \Cref{thm:move-event-from-freeable}, $\ahist\in\freeableof{\sigma.\anactp}{\anadrp}$ because $\historyof{\sigma.\anactp}=\historyof{\sigma}.\freeof{\anadr}$.
				This concludes the property.

				%%%%%%%%%%%%%%%%%%%%%%%%%%%%%%%%%%%%%%%%%%%%%%%%%%%%%%%%%%%
				%%%%%%%%%%%%%%%%%%%%%%%%%%%%%%%%%%%%%%%%%%%%%%%%%%%%%%%%%%%
				\ad{\Cref{proof:elision:goal:moreneq}}
				We have $\heapcomputof{\tau.\anact}{\validof{\tau}}=\heapcomputof{\tau}{\validof{\tau.\anact}}\subseteq\heapcomputof{\tau}{\validof{\tau}}$.
				Moreover, we have $\heapcomput{\tau}=\heapcomput{\tau.\anact}$ and $\heapcomput{\sigma}=\heapcomput{\sigma.\anactp}$.
				So the property follows \Cref{proof:elision:premise:moreneq}.

				%%%%%%%%%%%%%%%%%%%%%%%%%%%%%%%%%%%%%%%%%%%%%%%%%%%%%%%%%%%
				%%%%%%%%%%%%%%%%%%%%%%%%%%%%%%%%%%%%%%%%%%%%%%%%%%%%%%%%%%%
				\ad{\Cref{proof:elision:goal:retired-new}}
				By definition, we have \[
					\retiredof{\tau.\anact}=\retiredof{\tau}\setminus\set{\anadr}
					\qquad\text{and}\qquad
					\retiredof{\sigma.\anactp}=\retiredof{\sigma}\setminus\set{\anadr}
					\ .
				\]
				The claim follows from \Cref{proof:elision:premise:retired-new} thus.

				%%%%%%%%%%%%%%%%%%%%%%%%%%%%%%%%%%%%%%%%%%%%%%%%%%%%%%%%%%%
				%%%%%%%%%%%%%%%%%%%%%%%%%%%%%%%%%%%%%%%%%%%%%%%%%%%%%%%%%%%
				\ad{\Cref{proof:elision:goal:freed-not-retired}}
				We have $\freedof{\tau.\anact}=\freedof{\tau}\cup\set{\anadr}$ and $\retiredof{\tau.\anact}=\retiredof{\tau}\setminus\set{\anadr}$ by definition.
				Hence, the claim follows from \Cref{proof:elision:premise:freed-not-retired}.

				%%%%%%%%%%%%%%%%%%%%%%%%%%%%%%%%%%%%%%%%%%%%%%%%%%%%%%%%%%%
				%%%%%%%%%%%%%%%%%%%%%%%%%%%%%%%%%%%%%%%%%%%%%%%%%%%%%%%%%%%
				\ad{\Cref{proof:elision:goal:fresh}}
				Consider $\anadrp\in\freshof{\sigma.\anactp}$.
				Then, $\anadrp\in\freshof{\sigma}$.
				Let $\historyof{\tau}=\ahist$ and $\historyof{\sigma}=\ahistp$.
				We have $\historyof{\tau.\anact}=\ahist.\freeof{\anadr}$ and $\historyof{\sigma.\anactp}=\ahistp.\freeof{\anadr}$.
				Let $\ahistpp\in\freeableof{\sigma.\anactp}{\anadrp}$.
				Then, $\freeof{\anadr}.\ahistpp\in\freeableof{\ahistp}{\anadrp}$ by \Cref{thm:move-event-from-freeable}.
				By \Cref{proof:elision:premise:fresh} together with $\anadrp\in\freshof{\sigma}$, we have $\freeof{\anadr}.\ahistpp\in\freeableof{\ahist}{\anadrp}$.
				Again by \Cref{thm:move-event-from-freeable}, we get $\ahistpp\in\freeableof{\tau.\anact}{\anadrp}$.
				This concludes the claim.

		%=================================================================================================%
		%=================================================================================================%
		%=================================================================================================%
		%=================================================================================================%
				\item[$\acom\equiv\apvar:=\malloc$ and $\heapcomputof{\tau.\anact}{\apvar}=\anadr\in\freshof{\sigma}$]
				The update is $\anup=[\apvar\mapsto\anadr,\psel{\anadr}\mapsto\segval,\dsel{\anadr}\mapsto\advalue]$ with $\anadr\in\freshof{\tau}\cup\freedof{\tau}$.
				By case assumption, we can choose $\anupp=\anup$ and get that $\anactp$ is indeed enabled after $\sigma$.

				We first show two auxiliary statements:
				\begin{auxiliary}
					% \heapcomputof{\tau.\anact}{\validof{\tau}\setminus\set{\apvar}}&=\heapcomputof{\tau}{\validof{\tau}\setminus\set{\apvar}}
					\heapcomputof{\tau.\anact}{\validof{\tau.\anact}}&=\heapcomputof{\tau}{\validof{\tau}\setminus\set{\apvar,\psel{\anadr}}}\cup\set{\anadr}
					\label[aux]{proof:elision:malloc:valid-heap-tau}
					\\
					% \heapcomputof{\sigma.\anactp}{\validof{\sigma}\setminus\set{\apvar}}&=\heapcomputof{\sigma}{\validof{\sigma}\setminus\set{\apvar}}
					\heapcomputof{\sigma.\anact}{\validof{\sigma.\anact}}&=\heapcomputof{\sigma}{\validof{\sigma}\setminus\set{\apvar,\psel{\anadr}}}\cup\set{\anadr}
					\label[aux]{proof:elision:malloc:valid-heap-sigma}
				\end{auxiliary}

				%%%%%%%%%%%%%%%%%%%%%%%%%%%%%%%%%%%%%%%%%%%%%%%%%%%%%%%%%%%
				%%%%%%%%%%%%%%%%%%%%%%%%%%%%%%%%%%%%%%%%%%%%%%%%%%%%%%%%%%%
				\ad{\Cref{proof:elision:malloc:valid-heap-tau}}
				We conclude this property as follows:
				% Note that $\anact$ changes only the valuation of $\apvar$ and $\psel{\anadr}$.
				% And because $\anadr\in\freshof{\tau}\cup\freedof{\tau}$ we have $\psel{\anadr}\notin\validof{\tau}$ by \Cref{thm:fresh-not-valid,thm:free-not-valid}.
				% Moreover, we have $\validof{\tau.\anact}=\validof{\tau}\cup\set{\apvar,\psel{\anadr}}$.
				% So we conclude as follows:
				\begin{align*}
					\heapcomputof{\tau.\anact}{\validof{\tau.\anact}}
					=~&
					\heapcomputof{\tau.\anact}{\validof{\tau}\cup\set{\apvar,\psel{\anadr}}}
					\\=~&
					\heapcomputof{\tau.\anact}{\validof{\tau}\setminus\set{\apvar,\psel{\anadr}}}\cup\heapcomputof{\tau.\anact}{\set{\apvar,\psel{\anadr}}}
					\\=~&
					\heapcomputof{\tau}{\validof{\tau}\setminus\set{\apvar,\psel{\anadr}}}\cup\set{\anadr}
					\ .
				\end{align*}

				%%%%%%%%%%%%%%%%%%%%%%%%%%%%%%%%%%%%%%%%%%%%%%%%%%%%%%%%%%%
				%%%%%%%%%%%%%%%%%%%%%%%%%%%%%%%%%%%%%%%%%%%%%%%%%%%%%%%%%%%
				\ad{\Cref{proof:elision:malloc:valid-heap-sigma}}
				Analogous to \Cref{proof:elision:malloc:valid-heap-tau}.

				%%%%%%%%%%%%%%%%%%%%%%%%%%%%%%%%%%%%%%%%%%%%%%%%%%%%%%%%%%%
				%%%%%%%%%%%%%%%%%%%%%%%%%%%%%%%%%%%%%%%%%%%%%%%%%%%%%%%%%%%
				\ad{\Cref{proof:elision:goal:valid-heap}}
				\Cref{proof:elision:malloc:valid-heap-tau} with $\validof{\tau.\anact}=\validof{\tau}\cup\set{\apvar,\psel{\anadr}}$ gives the following:
				\begin{align*}
					&
					\domof{\restrict{\heapcomput{\tau.\anact}}{\validof{\tau.\anact}}}
					\\=~&
					\validof{\tau.\anact}\cup\dvars\cup\setcond{\dsel{\anadrp}}{\anadrp\in\heapcomputof{\tau.\anact}{\validof{\tau.\anact}}}
					\\=~&
					(\validof{\tau}\setminus\set{\apvar,\psel{\anadr}})\cup\set{\apvar,\psel{\anadr}}\cup\dvars\\~&\cup\setcond{\dsel{\anadrp}}{\anadrp\in\heapcomputof{\tau}{\validof{\tau}\setminus\set{\apvar,\psel{\anadr}}}}\cup\set{\dsel{\anadr}}
					\\=~&
					\domof{\restrict{\heapcomput{\tau}}{\validof{\tau}\setminus\set{\apvar,\psel{\anadr}}}}\cup\set{\apvar,\psel{\anadr},\dsel{\anadr}}
					\ .
				\end{align*}
				By definition then, we have:
				\begin{align*}
				 	\restrict{\heapcomput{\tau.\anact}}{\validof{\tau.\anact}}
				 	=~&
				 	(\restrict{\heapcomput{\tau}}{\validof{\tau}\setminus\set{\apvar,\psel{\anadr}}})[\apvar\mapsto\anadr,\psel{\anadr}\mapsto\segval,\dsel{\anadr}\mapsto\advalue]
				 	\\=~&
				 	(\restrict{(\restrict{\heapcomput{\tau}}{\validof{\tau}})}{\validof{\tau}\setminus\set{\apvar,\psel{\anadr}}})[\apvar\mapsto\anadr,\psel{\anadr}\mapsto\segval,\dsel{\anadr}\mapsto\advalue]
				 	\ .
				 	\intertext{
				Along the same lines, we get: 
				 	}
				 	\restrict{\heapcomput{\sigma.\anactp}}{\validof{\sigma.\anactp}}=~&(\restrict{(\restrict{\heapcomput{\sigma}}{\validof{\sigma}})}{\validof{\sigma}\setminus\set{\apvar,\psel{\anadr}}})[\apvar\mapsto\anadr,\psel{\anadr}\mapsto\segval,\dsel{\anadr}\mapsto\advalue]\ .
				\end{align*}
				By \Cref{proof:elision:premise:valid-heap,proof:elision:aux:valid} we have:
				\[\restrict{(\restrict{\heapcomput{\tau}}{\validof{\tau}})}{\validof{\tau}\setminus\set{\apvar,\psel{\anadr}}}=\restrict{(\restrict{\heapcomput{\sigma}}{\validof{\sigma}})}{\validof{\sigma}\setminus\set{\apvar,\psel{\anadr}}}\ .\]
				This concludes the claim.

				%%%%%%%%%%%%%%%%%%%%%%%%%%%%%%%%%%%%%%%%%%%%%%%%%%%%%%%%%%%
				%%%%%%%%%%%%%%%%%%%%%%%%%%%%%%%%%%%%%%%%%%%%%%%%%%%%%%%%%%%
				\ad{\Cref{proof:elision:goal:obsrel}}
				From \Cref{proof:elision:malloc:valid-heap-tau} and \Cref{thm:adrof-valid-heap-restriction} we get:
				\begin{align*}
					&\adrof{\restrict{\heapcomput{\tau.\anact}}{\validof{\tau.\anact}}}
					\\=~&
					(\validof{\tau.\anact}\cap\adr)\cup\heapcomputof{\tau.\anact}{\validof{\tau.\anact}}
					\\=~&
					((\validof{\tau}\cup\set{\apvar,\psel{\anadr}})\cap\adr)\cup
					\heapcomputof{\tau}{\validof{\tau}\setminus\set{\apvar,\psel{\anadr}}}\cup\set{\anadr}
					\\=~&
					(\validof{\tau}\cap\adr)\cup
					\heapcomputof{\tau}{\validof{\tau}\setminus\set{\apvar,\psel{\anadr}}}\cup\set{\anadr}
					\\\subseteq~&
					(\validof{\tau}\cap\adr)\cup\heapcomputof{\tau}{\validof{\tau}}\cup\set{\anadr}
					=
					\adrof{\restrict{\heapcomput{\tau}}{\validof{\tau}}}\cup\set{\anadr}
				\end{align*}
				We have $\freeableof{\tau.\anact}{\anadrp}=\freeableof{\tau}{\anadrp}$ and $\freeableof{\sigma.\anactp}{\anadrp}=\freeableof{\sigma}{\anadrp}$ for all $\anadrp\in\adr$ because $\anact$/$\anactp$ does not emit an event.
				By \Cref{proof:elision:premise:obsrel}, it remains to show that $\freeableof{\tau}{\anadr}\subseteq\freeableof{\sigma}{\anadr}$.
				This holds by \Cref{proof:elision:premise:fresh}.
				% By \Cref{proof:elision:premise:freed-not-retired} and \Cref{thm:disjoint-fresh-retired} we have $\anadr\notin\retiredof{\tau}$.
				% Hence, $\freeableof{\tau}{\anadr}\subseteq\freeableof{\sigma}{\anadr}$ follows from $\anadr\in\freshof{\sigma}$ together with elision support (\Cref{def:elision-support}\ref{def:elision-support:fresh-new}).
				% This concludes the claim.

				%%%%%%%%%%%%%%%%%%%%%%%%%%%%%%%%%%%%%%%%%%%%%%%%%%%%%%%%%%%
				%%%%%%%%%%%%%%%%%%%%%%%%%%%%%%%%%%%%%%%%%%%%%%%%%%%%%%%%%%%
				\ad{\Cref{proof:elision:goal:moreneq}}
				Consider $\anexp,\anexpp\in\pvars\cup\setcond{\psel{\anadr},\dsel{\anadr}}{\anadr\in\heapcomputof{\tau.\anact}{\validof{\tau.\anact}}}$ with $\heapcomputof{\tau.\anact}{\anexp}\neq\heapcomputof{\tau.\anact}{\anexpp}$.
				We have already shown that $\adrof{\restrict{\heapcomput{\tau.\anact}}{\validof{\tau.\anact}}}\subseteq\adrof{\restrict{\heapcomput{\tau}}{\validof{\tau}}}\cup\set{\anadr}$ holds for \Cref{proof:elision:goal:obsrel} above.
				So we get: \[\anexp,\anexpp\in\pvars\cup\setcond{\psel{\anadr}}{\anadr\in\heapcomputof{\tau}{\validof{\tau}}}\cup\set{\psel{\anadr}}\ .\]
				We do a case distinction on $\anexp,\anexpp$.
				\begin{compactitem}
					\item
					Consider $\anexp=\apvar$ and $\anexpp=\psel{\anadr}$.
					Then, $\heapcomputof{\sigma.\anactp}{\anexp}=\anadr\neq\segval=\heapcomputof{\sigma.\anactp}{\anexpp}$.

					\item
					Consider $\anexp=\psel{\anadr}$ and $\anexpp=\apvar$.
					Similar to the previous case.

					\item
					Consider $\anexp=\apvar$ and $\anexpp\neq\psel{\anadr}$.
					We have $\heapcomputof{\sigma.\anactp}{\apvar}=\anadr$.
					Since $\anadr\in\freshof{\sigma}$, we must have $\anadr\neq\heapcomputof{\sigma}{\anexpp}=\heapcomputof{\sigma.\anactp}{\anexpp}$ by \Cref{thm:fresh-notin-range}.

					\item
					Consider $\anexpp=\apvar$ and $\anexp\neq\psel{\anadr}$.
					Similar to the previous case.

					\item
					Consider $\anexp=\psel{\anadr}$ and $\anexpp\neq\apvar$.
					We have $\heapcomputof{\sigma.\anactp}{\psel{\anadr}}=\segval$.
					If $\heapcomputof{\sigma.\anactp}{\anexpp}=\segval$, then we $\anexpp\in\validof{\sigma.\anactp}$.
					By \Cref{proof:elision:goal:valid-heap} this gives $\heapcomputof{\tau.\anact}{\anexpp}=\heapcomputof{\sigma.\anactp}{\anexpp}$.
					Moreover, we have $\heapcomputof{\tau.\anact}{\psel{\anadr}}=\heapcomputof{\sigma.\anactp}{\psel{\anadr}}$.
					This contradicts the choice of $\anexp,\anexpp$.
					Hence, we must have $\heapcomputof{\sigma.\anactp}{\anexpp}\neq\segval=\heapcomputof{\sigma.\anactp}{\anexp}$ as desired.

					\item
					Consider $\anexpp=\psel{\anadr}$ and $\anexp\neq\apvar$.
					Similar to the previous case.

					\item
					Consider $\anexp,\anexpp\notin\set{\apvar,\psel{\anadr}}$.
					Then, $\heapcomputof{\tau}{\anexp}=\heapcomputof{\tau.\anact}{\anexp}$ and $\heapcomputof{\sigma}{\anexp}=\heapcomputof{\sigma.\anactp}{\anexp}$.
					Similarly, $\heapcomputof{\tau}{\anexpp}=\heapcomputof{\tau.\anact}{\anexpp}$ and $\heapcomputof{\sigma}{\anexpp}=\heapcomputof{\sigma.\anactp}{\anexpp}$.
					So \Cref{proof:elision:premise:moreneq} yields $\heapcomputof{\sigma.\anactp}{\anexp}\neq\heapcomputof{\sigma.\anactp}{\anexpp}$.
				\end{compactitem}
				The above case distinction is complete.
				This concludes \Cref{proof:elision:goal:moreneq}.

				%%%%%%%%%%%%%%%%%%%%%%%%%%%%%%%%%%%%%%%%%%%%%%%%%%%%%%%%%%%
				%%%%%%%%%%%%%%%%%%%%%%%%%%%%%%%%%%%%%%%%%%%%%%%%%%%%%%%%%%%
				\ad{\Cref{proof:elision:goal:retired-new}}
				We have $\retiredof{\tau}=\retiredof{\tau.\anact}$ and $\retiredof{\sigma}=\retiredof{\sigma.\anact}$ by definition.
				The claim follows from \Cref{proof:elision:premise:retired-new} thus.

				%%%%%%%%%%%%%%%%%%%%%%%%%%%%%%%%%%%%%%%%%%%%%%%%%%%%%%%%%%%
				%%%%%%%%%%%%%%%%%%%%%%%%%%%%%%%%%%%%%%%%%%%%%%%%%%%%%%%%%%%
				\ad{\Cref{proof:elision:goal:freed-not-retired}}
				We have $\retiredof{\tau.\anact}=\retiredof{\tau}$ and $\freedof{\tau.\anact}=\freedof{\tau}\setminus\set{\anadr}$.
				Hence, the claim follows from \Cref{proof:elision:premise:freed-not-retired}

				%%%%%%%%%%%%%%%%%%%%%%%%%%%%%%%%%%%%%%%%%%%%%%%%%%%%%%%%%%%
				%%%%%%%%%%%%%%%%%%%%%%%%%%%%%%%%%%%%%%%%%%%%%%%%%%%%%%%%%%%
				\ad{\Cref{proof:elision:goal:fresh}}
				Follows immediately from \Cref{proof:elision:premise:fresh} together with $\historyof{\sigma.\anactp}=\historyof{\sigma}$ and $\freshof{\sigma.\anactp}\subseteq\freshof{\sigma}$.

			\end{casedistinction}

		%=================================================================================================%
		%=================================================================================================%
		%=================================================================================================%
		%=================================================================================================%
			\medskip
			The above case distinction handles all cases but:
			\begin{compactitem}
				\item $\acom\equiv\freeof{\anadr}$ with $\historyof{\sigma}.\freeof{\anadr}\notin\specof{\smrobs}$
				\item $\acom\equiv\apvar:=\malloc$ with $\heapcomputof{\tau.\anact}{\apvar}=\anadr\notin\freshof{\sigma}$
			\end{compactitem}
			In these cases we cannot find an appropriate $\anactp$ as before.
			\smallskip

			\begin{casedistinction}
		%=================================================================================================%
		%=================================================================================================%
		%=================================================================================================%
		%=================================================================================================%
				\item[$\acom\equiv\freeof{\anadr}$ and $\historyof{\sigma}.\freeof{\anadr}\notin\specof{\smrobs}$]
				We show that $\sigma$ already has the required properties.
				That is, we do not need to mimic $\anact$.
				Note that we have $\freeof{\anadr}\notin\freeableof{\sigma}{\anadr}$.
				Hence, $\anadr\notin\vadrof{\tau}$ must hold by \Cref{proof:elision:premise:obsrel}.
				We now show that $\sigma$ has the desired properties.

				%%%%%%%%%%%%%%%%%%%%%%%%%%%%%%%%%%%%%%%%%%%%%%%%%%%%%%%%%%%
				%%%%%%%%%%%%%%%%%%%%%%%%%%%%%%%%%%%%%%%%%%%%%%%%%%%%%%%%%%%
				\ad{$\tau.\anact\computequiv\sigma$}
				By definition, $\controlof{\tau.\anact}=\controlof{\tau}$.
				Hence, $\controlof{\tau.\anact}=\controlof{\sigma}$ follows from \Cref{proof:elision:premise:control}.
				It remains to show $\restrict{\heapcomput{\tau.\anact}}{\validof{\tau.\anact}}=\restrict{\heapcomput{\sigma}}{\validof{\sigma}}$.
				By \Cref{proof:elision:premise:valid-heap}, it suffices to show $\restrict{\heapcomput{\tau}}{\validof{\tau}}=\restrict{\heapcomput{\tau.\anact}}{\validof{\tau.\anact}}$.
				To arrive at this equality, we first show $\validof{\tau}=\validof{\tau.\anact}$.
				The inclusion from right to left, $\validof{\tau.\anact}\subseteq\validof{\tau}$, holds by definition.
				To see the reverse direction, $\validof{\tau}\subseteq\validof{\tau.\anact}$, consider $\apexp\in\validof{\tau}$.
				Then, $\apexp\not\equiv\psel{\anadr}$ must hold as for otherwise we had $\anadr\in\adrof{\restrict{\heapcomput{\tau}}{\validof{\tau}}}$ which does not hold as argued before.
				Moreover, $\heapcomputof{\tau}{\apexp}\neq\anadr$ must hold as for otherwise we would again get $\anadr\in\adrof{\restrict{\heapcomput{\tau}}{\validof{\tau}}}$.
				Hence, by the definition of validity, we have $\apexp\in\validof{\tau.\anact}$.
				With this we can conclude immediately by $\restrict{\heapcomput{\tau.\anact}}{\validof{\tau.\anact}}=\restrict{\heapcomput{\tau}}{\validof{\tau.\anact}}=\restrict{\heapcomput{\tau}}{\validof{\tau}}$ where the first equality is due to $\heapcomput{\tau}=\heapcomput{\tau.\anact}$ and the second equality is due to $\validof{\tau}=\validof{\tau.\anact}$.

				%%%%%%%%%%%%%%%%%%%%%%%%%%%%%%%%%%%%%%%%%%%%%%%%%%%%%%%%%%%
				%%%%%%%%%%%%%%%%%%%%%%%%%%%%%%%%%%%%%%%%%%%%%%%%%%%%%%%%%%%
				\ad{$\tau.\anact\obsrel\sigma$}
				Let $\anadrp\in\adrof{\restrict{\heapcomput{\tau.\anact}}{\validof{\tau.\anact}}}$.
				We get $\anadrp\in\adrof{\restrict{\heapcomput{\tau}}{\validof{\tau}}}$.
				This means $\anadr\neq\anadrp$ due to the above.
				Moreover, by \Cref{proof:elision:premise:obsrel} we have $\freeableof{\tau}{\anadrp}\subseteq\freeableof{\sigma}{\anadrp}$.
				So it suffices to show that $\freeableof{\tau}{\anadrp}=\freeableof{\tau.\anact}{\anadrp}$ holds.
				This holds because $\anobs$ supports elision (\Cref{def:elision-support}\ref{def:elision-support:frees}) by assumption.
				This concludes the property.

				%%%%%%%%%%%%%%%%%%%%%%%%%%%%%%%%%%%%%%%%%%%%%%%%%%%%%%%%%%%
				%%%%%%%%%%%%%%%%%%%%%%%%%%%%%%%%%%%%%%%%%%%%%%%%%%%%%%%%%%%
				\ad{remaining properties}
				It remains to establish \Cref{proof:elision:goal:moreneq,proof:elision:goal:retired-new,proof:elision:goal:freed-not-retired,proof:elision:goal:fresh}.
				By definition, we have $\heapcomputof{\tau.\anact}{\validof{\tau}}=\heapcomputof{\tau}{\validof{\tau.\anact}}\subseteq\heapcomputof{\tau}{\validof{\tau}}$.
				Moreover, $\heapcomput{\tau}=\heapcomput{\tau.\anact}$.
				So \Cref{proof:elision:goal:moreneq} follows by \Cref{proof:elision:premise:moreneq}.
				Furthermore, we have $\retiredof{\tau.\anact}=\retiredof{\tau}\setminus\set{\anadr}$.
				Thus, \Cref{proof:elision:goal:retired-new} follows by \Cref{proof:elision:premise:retired-new}.
				And because $\freedof{\tau.\anact}=\freedof{\tau}\cup\set{\anadr}$ we get \Cref{proof:elision:goal:freed-not-retired} follows from \Cref{proof:elision:premise:freed-not-retired}.
				To see the remaining \Cref{proof:elision:goal:fresh}, consider some $\anadrp\in\freshof{\sigma}$.
				By assumption, $\anadrp\neq\anadr$ must hold because $\freeof{\anadr}$ is not enabled after $\sigma$ but enabled after $\tau$.
				Hence, \Cref{def:elision-support}\ref{def:elision-support:frees} gives $\freeableof{\tau.\anact}{\anadrp}=\freeableof{\tau}{\anadrp}$.
				So by \Cref{proof:elision:premise:fresh} we get the desired $\freeableof{\tau.\anact}{\anadrp}=\freeableof{\tau}{\anadrp}\subseteq\freeableof{\sigma}{\anadrp}$.

		%=================================================================================================%
		%=================================================================================================%
		%=================================================================================================%
		%=================================================================================================%
				\item[$\acom\equiv\apvar:=\malloc$ and $\heapcomputof{\tau.\anact}{\apvar}=\anadr\notin\freshof{\sigma}$]
				\Cref{thm:replacing-addresses-in-computations-new} yields $\gamma\in\freesemobs$ and $\anadrp\in\adr$ with the following properties:
				\begin{compactitem}
					\item $\sigma\computequiv\gamma$ and $\sigma\obsrel\gamma$,
					\item $\retiredof{\sigma}\subseteq\retiredof{\gamma}\cup\set{\anadr}$,
					\item $\anadr\in\freshof{\gamma}$ and $\anadrp\in\freshof{\sigma}\cap\freshof{\tau}$,
					\item $\anadrp\in\freshof{\sigma}\iff\anadr\in\freshof{\tau}$ and $\freshof{\sigma}\setminus\set{\anadr,\anadrp}=\freshof{\tau}\setminus\set{\anadr,\anadrp}$,
					\item $\renamingof{\freeableof{\sigma}{\anadrp}}{\anadrp}{\anadr}=\freeableof{\gamma}{\anadr}$ and $\freeableof{\sigma}{\anadrpp}=\freeableof{\gamma}{\anadrpp}$ for any address $\anadr\neq\anadrpp\neq\anadr$, and
					\item for all $\anexp,\anexpp\in\pvars\cup\setcond{\psel{\anadrpp},\dsel{\anadrpp}}{\anadrpp\in\heapcomputof{\sigma}{\validof{\sigma}}}$ we have $\heapcomputof{\sigma}{\anexp}\neq\heapcomputof{\sigma}{\anexpp}$ implies $\heapcomputof{\gamma}{\anexp}\neq\heapcomputof{\gamma}{\anexpp}$.
				\end{compactitem}
				% \Cref{thm:replacing-addresses-in-computations-new} yields $\gamma$ with $\sigma\computequiv\gamma$, $\sigma\obsrel\gamma$, $\anadr\in\freshof{\gamma}$, and $\retiredof{\sigma}\subseteq\retiredof{\gamma}\cup\set{\anadr}$.
				% And there is $\anadrp\in\freshof{\sigma}\cap\freshof{\tau}$ such that $\freeableof{\sigma}{\anadr}=\renamingof{\freeableof{\gamma}{\anadrp}}{\anadrp}{\anadr}$, $\freeableof{\sigma}{\anadrp}=\renamingof{\freeableof{\gamma}{\anadr}}{\anadr}{\anadrp}$, and $\freeableof{\sigma}{\anadrpp}=\freeableof{\gamma}{\anadrpp}$ for any address $\anadr\neq\anadrpp\neq\anadr$.
				% Moreover, for all $\anexp,\anexpp\in\pvars\cup\setcond{\psel{\anadr},\dsel{\anadr}}{\anadr\in\heapcomputof{\sigma}{\validof{\sigma}}}$ we have $\heapcomputof{\sigma}{\anexp}\neq\heapcomputof{\sigma}{\anexpp}$ implies $\heapcomputof{\gamma}{\anexp}\neq\heapcomputof{\gamma}{\anexpp}$.
				Hence, \Cref{proof:elision:premise:control,proof:elision:premise:valid-heap,proof:elision:premise:obsrel,proof:elision:premise:moreneq,proof:elision:premise:retired-new,proof:elision:premise:freed-not-retired} hold for $\tau$ and $\gamma$, that is:
				\begin{compactitem}
					\item $\controlof{\tau}=\controlof{\gamma}$
					\item $\restrict{\heapcomput{\tau}}{\validof{\tau}}=\restrict{\heapcomput{\gamma}}{\validof{\gamma}}$
					\item $\forall\anadr\in\vadrof{\tau}.~\freeableof{\tau}{\anadr}\subseteq\freeableof{\gamma}{\anadr}$
					\item $\forall\anexp,\anexpp\in\pvars\cup\setcond{\psel{\anadr}}{\anadr\in\heapcomputof{\tau}{\validof{\tau}}}.~\heapcomputof{\tau}{\anexp}\neq\heapcomputof{\tau}{\anexpp}\implies\heapcomputof{\gamma}{\anexp}\neq\heapcomputof{\gamma}{\anexpp}$
					\item $\freedof{\tau}\cap\retiredof{\tau}=\emptyset$
					\item $\retiredof{\tau}\subseteq\retiredof{\gamma}$
					\item $\forall\anadr\in\freshof{\gamma}.~\freeableof{\tau}{\anadr}\subseteq\freeableof{\gamma}{\anadr}$
				\end{compactitem}
				For the second to last property, we have to show that $\anadr\notin\retiredof{\tau}$ due to \Cref{proof:elision:premise:retired-new}.
				By definition, we have $\anadr\in\freshof{\tau}\cup\freedof{\tau}$.
				Hence, \Cref{proof:elision:premise:freed-not-retired} together with \Cref{thm:disjoint-fresh-retired} yields the desired $\anadr\notin\retiredof{\tau}$.

				For the last property, consider some $\anadrpp\in\freshof{\gamma}$.
				If $\anadr\neq\anadrpp\neq\anadrp$, then we have $\anadrpp\in\freshof{\sigma}$ and $\freeableof{\tau}{\anadrpp}\subseteq\freeableof{\sigma}{\anadrpp}=\freeableof{\gamma}{\anadrpp}$.
				It remains to consider $\anadrpp\in\set{\anadr,\anadrp}$.
				Recall that we have $\anadr\notin\freshof{\sigma}$ by assumption.
				Hence, $\anadrp\notin\freshof{\gamma}$ according to our invocation of \Cref{thm:replacing-addresses-in-computations-new} above.
				That is, $\anadrp=\anadrpp$ cannot occur.
				So consider the remaining case: $\anadrpp=\anadr$.
				Note that $\anadrp\in\freshof{\sigma}$ and $\anadrp\in\freshof{\tau}$ hold.
				We have:
				\begin{align*}
					\freeableof{\tau}{\anadr}
					\subseteq
					\renamingof{\freeableof{\tau}{\anadrp}}{\anadrp}{\anadr}
					\subseteq
					\renamingof{\freeableof{\sigma}{\anadrp}}{\anadrp}{\anadr}
					\subseteq
					\freeableof{\gamma}{\anadr}
				\end{align*}
				where the first inclusion is due to \Cref{thm:elision-support-lift}, the second inclusion is due to \Cref{proof:elision:premise:fresh}, and the last inclusion holds due to the properties of $\gamma$ listed above.

				Now, we repeat the induction step for $\tau.\anact$ and $\gamma$.
				Then, the previous $\malloc$ case from above will apply.
				That is, we identify some $\anactp$ such that $\gamma.\anactp$ has the desired properties.
			\end{casedistinction}
	\end{description}
	This concludes the claim.
\end{proof}
