# Supplementary material for: Pointer Life Cycle Types for Lock-Free Data Structures with Memory Reclamation
Source: arXiv:1910.11714 source file (2019-11-26)
Supplement: Supplementary file 3 [file synthesis.tex]

%!TEX root = ../main.tex

\subsection{Synthesis}

\todoi{use the new macro $\apavar$ for pointers and angles}

\begin{definition}
	Let $\aninstantiation$ be some type instantiation.
	We say that a type $\atype$ stems from $\aninstantiation$, denoted by $\atype\typefrom\aninstantiation$, if the custom guarantees it contains are from $\aninstantiation$, that is, if $\atype\subseteq\set{\gactive,\glocal,\gsafeaccess}\cup\aninstantiation$ holds.
	For a type environment $\env$ we write $\env\envfrom\aninstantiation$ if $\env(\apavar)\typefrom\aninstantiation$ for all $\apavar\in\domof{\env}$.
	We denote type inference wrt. to $\aninstantiation$ by $\checkof[\aninstantiation]{\env}{\anevent}{\envp}$.
	Similarly, $\typejudge[\aninstantiation]{\env}{\astmt}{\envp}$ denotes a type derivation wrt. to $\aninstantiation$.
	% Similarly, $\typechecks[\aninstantiation]{\aprog}$ denotes a type check of program $\aprog$ wrt. to $\aninstantiation$.
\end{definition}

% \begin{assumption}
% 	\label{assumption:isprotected-reach}
% 	Let $L_\mathit{final}$ be the final locations of $\smrobs$.
% 	Then, we assume:
% 	\[ \forall\ahist.~~ \isprotectedof{\athread}{\anadr}{\ahist} \iff \lreachof{\athread}{\anadr}{\set{\ahist}}\cap L_\mathit{final} \neq \emptyset \ . \]
% \end{assumption}

\begin{assumption}
	\label{assumption:isprotected-reach-new-new}
	Let $L_\mathit{final}$ be the final locations of $\anobs$.
	Then, we assume: \sw{as def to use if needed?}
	\[ \forall\athread,\anadr,\ahist.~~ \ahist\in\typehistof{\athread}{\anadr}{\gsafeaccess} \implies \lreachof{\athread}{\anadr}{\set{\ahist.\freeof{\anadr}}}\subseteq L_\mathit{final} \ . \]
\end{assumption}

\begin{assumption}
	\label{assumption:bounded-precision}
	Consider some SMR automaton $\anobs$ and some type instantiation $\aninstantiation$.
	Let $\atype\subseteq\aninstantiation$.
	Then we assume:
	\[
		\forall\ahist,\athread,\anadr.~
		\lreachof{\athread}{\anadr}{\set{\ahist}}\cap\lreachof{\athread}{\anadr}{\typehistof{\athread}{\anadr}{\atype}}
		\implies
		\ahist\in\typehistof{\athread}{\anadr}{\atype}
		\ .
	\]
\end{assumption}

\begin{definition}
	\label{def:lessprecise}
	A type $\atypep$ is more or equally precise than another type $\atype$, denoted by $\atype\lessprecise\atypep$, if
	\begin{align*}
		\atype\cap\set{\gactive,\glocal,\gsafeaccess}=\atypep\cap\set{\gactive,\glocal,\gsafeaccess}
		\qquad\text{and}\qquad
		\forall\athread,\anadr.~~
		\typehistof{\athread}{\anadr}{\atypep}
		\subseteq
		\typehistof{\athread}{\anadr}{\atype}
		\ .
	\end{align*}
	Then, $\env\lessprecise\envp$ if $\domof{\env}\subseteq\domof{\envp}$ and $\env(\apavar)\lessprecise\envp(\apavar)$ for all $\apavar\in\domof{\env}$.
\end{definition}

\begin{definition}
	\label{def:mostprecise-new}
	A type instantiation $\aninstantiation$ is \emph{most precise} if:
	\begin{align*}
		\forall\,\atype\typefrom\aninstantiation~
		\forall\apavar,\acom~
		\exists\,G\subseteq\aninstantiation~
		% \forall\athread,\anadr,\ahist.~~&
		\forall\athread,\anadr.~~&
		\lreachof{\athread}{\anadr}{\typehistof{\athread}{\anadr}{G}}
		=
		\lclosureof{\lpostof{\apavar}{\acom}{\lreachof{\athread}{\anadr}{\typehistof{\athread}{\anadr}{\atype}}}}
		% \\
		% \wedge~&
		% \lreachof{\athread}{\anadr}{\typehistof{\athread}{\anadr}{G}}
		% \cap
		% \lreachof{\athread}{\anadr}{\set{\ahist}}
		% \neq\emptyset
		% \implies
		% \ahist\in\typehistof{\athread}{\anadr}{G}
		\ .
	\end{align*}
\end{definition}

% \begin{lemma}
% 	\label{thm:intersection-vs-lclosure-new}
% 	Function $\lclosure$ is monotone:
% 	$L\subseteq L'$ implies $\lclosureof{L}\subseteq\lclosureof{L'}$.
% \end{lemma}

% \begin{lemma}
% 	\label{thm:intersection-vs-lpost-new}
% 	Function $\lpost$ is monotone:
% 	$L\subseteq L'$ implies $\lpostof{\apavar}{\acom}{L}\subseteq\lpostof{\apavar}{\acom}{L'}$.
% \end{lemma}

\begin{lemma}
	\label{thm:lessprecise-vs-gactive-removal}
	Let $\atype\lessprecise\atypep$.
	Then, $\atype\setminus\set{\gactive}\lessprecise\atypep\setminus\set{\gactive}$.
\end{lemma}

\begin{lemma}
	\label{thm:lessprecise-reach-inclusion-WRONG}
	If $\envi\lessprecise\env$ then $\lreachof{\athread}{\anadr}{\typehistof{\athread}{\anadr}{\env(\apavar)}}\subseteq\lreachof{\athread}{\anadr}{\typehistof{\athread}{\anadr}{\envi(\apavar)}}$ for all $\athread,\anadr,\apavar$.
\end{lemma}

\begin{lemma}
	\label{thm:unpealing}
	Consider some $\alocation,\apavar,\acom,\athread,\anadr,H$ with $\alocation\in\lclosureof{\lpostof{\apavar}{\acom}{\lreachof{\athread}{\anadr}{H}}}$.
	Then there are some $\alocation_1,\alocation_2,\varphi,\agenheap,\ahist_1,\ahist_2,\anevent$ with:
	\begin{align*}
		&\alocation_1\in\lreachof{\athread}{\anadr}{H}
		\quad\text{and}\quad
		\anevent=\evalcom{\agenheap}{\athread}{\acom}
		\quad\text{and}\quad
		% \psi(\apavar)=\anadr
		\quad\text{and}\quad
		\project{\ahist_2}{\athread}=\epsilon
		\\\text{and}\quad
		&\varphi=\set{\anovar\mapsto\athread,\anovarp\mapsto\anadr}
		\quad\text{and}\quad
		(\alocation_\mathit{init},\varphi)\trans{\ahist_1}(\alocation_1,\varphi)\trans{\anevent}(\alocation_2,\varphi)\trans{\ahist_2}(\alocation,\varphi)
		\\\text{and}\quad
		&\apavar\in\pvars\implies\anadr=\agenheap(\apavar)
		\quad\text{and}\quad
		\apavar\in\gvars\implies\anadr\in\agenheap(\apavar)
		\ .
	\end{align*}
\end{lemma}

\begin{lemma}
	\label{thm:gactive-through-locations}
	Let $\ahist,\ahistp,\anevent,\athread,\anadr,\alocation$ with $\set{\ahist,\ahist.\anevent,\ahistp}\subseteq\typehistof{\athread}{\anadr}{\gactive}$ and $\alocation\in\lreachof{\athread}{\anadr}{\set{\ahist}}\cap\lreachof{\athread}{\anadr}{\set{\ahistp}}$.
	Then, $\ahistp.\anevent\in\typehistof{\athread}{\anadr}{\gactive}$.
\end{lemma}

\begin{lemma}
	\label{thm:glocal-through-locations}
	Let $\ahist,\ahistp,\anevent,\athread,\anadr,\alocation$ with $\set{\ahist,\ahist.\anevent,\ahistp}\subseteq\typehistof{\athread}{\anadr}{\glocal}$ and $\alocation\in\lreachof{\athread}{\anadr}{\set{\ahist}}\cap\lreachof{\athread}{\anadr}{\set{\ahistp}}$.
	Then, $\ahistp.\anevent\in\typehistof{\athread}{\anadr}{\glocal}$.
\end{lemma}

\begin{lemma}
	\label{thm:gsafeaccess-through-locations}
	Consider some $\ahist,\ahistp,\athread,\anadr,\alocation$ such that $\ahist\in\typehistof{\athread}{\anadr}{\gsafeaccess}$ and $\alocation\in\lreachof{\athread}{\anadr}{\set{\ahist}}\cap\lreachof{\athread}{\anadr}{\set{\ahistp}}$.
	Then, $\ahistp\in\typehistof{\athread}{\anadr}{\gsafeaccess}$.
\end{lemma}

\begin{lemma}
	\label{thm:most-precise-mimicks-inference}
	Let $\envi_1,\envi_2\envfrom\aninstantiation$ and $\acom$ with $\checkof[\aninstantiation]{\envi_1}{\acom}{\envi_2}$.
	Let $\env_1\envfrom\aninstantiationp$ with $\envi_1\lessprecise\env_1$.
	If $\aninstantiationp$ is most precise, then there is $\env_2\envfrom\aninstantiationp$ such that $\checkof[\aninstantiationp]{\env_1}{\acom}{\env_2}$ and $\envi_2\lessprecise\env_2$.
\end{lemma}

\begin{lemma}
	\label{thm:most-precise-mimicks-judgements-com}
	Consider $\envi_1,\env_2\envfrom\aninstantiation$ and $\acom$ with $\typecom{\envi_1}{\acom}{\envi_2}$.
	Let $\env_1\envfrom\aninstantiationp$ with $\envi_1\lessprecise\env_1$.
	If $\aninstantiationp$ is most precise, then there is $\env_2\in\aninstantiationp$ such that $\typecom{\env_1}{\acom}{\env_2}$ and $\envi_2\lessprecise\env_2$.
\end{lemma}

\begin{lemma}
	\label{thm:most-precise-mimicks-judgements-stmt}
	Consider $\envi_1,\envi_2\envfrom\aninstantiation$ and $\astmt$ with $\typestmt{\envi_1}{\astmt}{\envi_2}$.
	Let $\env_1\envfrom\aninstantiationp$ with $\envi_1\lessprecise\env_1$.
	If $\aninstantiationp$ is most precise, then there is $\env_2\in\aninstantiationp$ such that $\typestmt{\env_1}{\astmt}{\env_2}$ and $\envi_2\lessprecise\env_2$.
\end{lemma}

\begin{lemma}
	\label{thm:most-precise-mimicks-typecheck}
	Consider $\aninstantiation,\aninstantiationp$ and $\aprog$ with $\typechecks[\aninstantiation]{\aprog}$.
	If $\aninstantiationp$ is most precise, then $\typechecks[\aninstantiationp]{\aprog}$.
\end{lemma}

\begin{lemma}
	\label{thm:synthesized-types-are-most-precise-new-new}
	Let $\aninstantiationp=\setcond{\gcustom{L}}{L\subseteq\lsetsetlfp}$ be the synthesized type system instantiation from \Cref{sec:synthesis}.
	Let $\anobs$ be deterministic.
	Then, $\aninstantiationp$ is most precise.
	\sw{fixed point solution relative to $\anobs$?}
\end{lemma}
