# Supplementary material for: Pointer Life Cycle Types for Lock-Free Data Structures with Memory Reclamation
Source: arXiv:1910.11714 source file (2019-11-26)
Supplement: Supplementary file 4 [file synthesis_proofs.tex]

%!TEX root = ../main.tex

\presection
\subsection{Synthesis}

\begin{proof}[Proof of \Cref{thm:intersection-vs-lclosure-new}]
	Follows from definition.
\end{proof}

\begin{proof}[Proof of \Cref{thm:intersection-vs-lpost-new}]
	Follows from definition.
\end{proof}

\begin{proof}[Proof of \Cref{thm:lessprecise-vs-gactive-removal}]
	Consider some types $\atype,\atypep$ with $\atype\lessprecise\atypep$.
	We show that $\atype\setminus\set{\gactive}\lessprecise\atypep\setminus\set{\gactive}$ holds.
	We immediately get the following:
	\begin{align*}
		(\atype\setminus\set{\gactive})\cap\set{\gactive,\glocal,\gsafeaccess}
		=(\atype\cap\set{\gactive,\glocal,\gsafeaccess})\setminus\set{\gactive}\:
		&=(\atypep\cap\set{\gactive,\glocal,\gsafeaccess})\setminus\set{\gactive}
		=(\atypep\setminus\set{\gactive})\cap\set{\gactive,\glocal,\gsafeaccess}
	\intertext{%
	where the first and last equalities are due to set theory and the second one is due to $\atype\lessprecise\atypep$.
	The remaining property follows similarly:
	}
		\lreachof{\athread}{\anadr}{\typehistof{\athread}{\anadr}{(\atypep\setminus\set{\gactive})\setminus\set{\gactive,\glocal,\gsafeaccess}}}\:
		&=
		\lreachof{\athread}{\anadr}{\typehistof{\athread}{\anadr}{\atypep\setminus\set{\gactive,\glocal,\gsafeaccess}}}\\
		&\subseteq
		\lreachof{\athread}{\anadr}{\typehistof{\athread}{\anadr}{\atype\setminus\set{\gactive,\glocal,\gsafeaccess}}}\\
		&=
		\lreachof{\athread}{\anadr}{\typehistof{\athread}{\anadr}{(\atype\setminus\set{\gactive})\setminus\set{\gactive,\glocal,\gsafeaccess}}}
		\ .
	\end{align*}
	This concludes the claim.
\end{proof}

\begin{proof}[Proof of \Cref{thm:lessprecise-reach-inclusion-WRONG}]
	Let $\envi\lessprecise\env$.
	Consider some $\apavar,\athread,\anadr,\alocation$ with $\alocation\in\lreachof{\athread}{\anadr}{\typehistof{\athread}{\anadr}{\env(\apavar)}}$.
	By definition, $\alocation\in\lreachof{\athread}{\anadr}{\typehistof{\athread}{\anadr}{\env(\apavar)\setminus\set{\gactive,\glocal,\gsafeaccess}}}$ and $\alocation\in\lreachof{\athread}{\anadr}{\typehistof{\athread}{\anadr}{\env(\apavar)\cap\set{\gactive,\glocal,\gsafeaccess}}}$.
	Due to the premise, $\envi\lessprecise\env$, we get $\alocation\in\lreachof{\athread}{\anadr}{\typehistof{\athread}{\anadr}{\envi(\apavar)\setminus\set{\gactive,\glocal,\gsafeaccess}}}$ and $\alocation\in\lreachof{\athread}{\anadr}{\typehistof{\athread}{\anadr}{\envi(\apavar)\cap\set{\gactive,\glocal,\gsafeaccess}}}$.
	Hence $\alocation\in\lreachof{\athread}{\anadr}{\typehistof{\athread}{\anadr}{\envi(\apavar)}}$.
	This concludes the claim.
	\todoi{the last implication does not hold}
\end{proof}

\begin{proof}[Proof of \Cref{thm:unpealing}]
	We need the following auxiliary result:
	for all $\alocation,\alocation',\varphi,\ahist,\anadr,\anadr',\athread,\athread'$ we have
	\begin{align}
		(\alocation,\varphi)\trans{\ahist}(\alocation',\varphi)\iff(\alocation,\renamingof{\renamingof{\varphi}{\athread}{\athread'}}{\anadr}{\anadr'})\trans{\renamingof{\renamingof{\ahist}{\athread}{\athread'}}{\anadr}{\anadr'}}(\alocation',\renamingof{\renamingof{\varphi}{\athread}{\athread'}}{\anadr}{\anadr'})
		\label[property]{proof:unpealing:renaming-vs-runs}
	\end{align}
	where $(\renamingof{\renamingof{\varphi}{\athread}{\athread'}}{\anadr}{\anadr'})(\anovar)=(\renamingof{\renamingof{\varphi(\anovar)}{\athread}{\athread'}}{\anadr}{\anadr'})$ and similarly for $\anovarp$.
	The above property follows from \cite[Lemma D.24]{DBLP:journals/corr/MeyerW19}. % poplref={thm:swaphist-versus-observerruns}

	Wlog. assume $\apavar\in\pvars$.
	The case for $\apavar\in\gvars$ is analogous.
	Towards the main result, let $\alocation_3\in\lclosureof{\lpostof{\apavar}{\acom}{\lreachof{\athread}{\anadr}{H}}}$.
	By definition, there is $\alocation_2,\varphi_2,\ahist_2'$ with:
	\begin{align}
		\alocation_2\in\lpostof{\apavar}{\acom}{\lreachof{\athread}{\anadr}{H}}
		\quad\text{and}\quad
		\project{\ahist_2'}{\varphi_2(\anovar)}=\epsilon
		\quad\text{and}\quad
		(\alocation_2,\varphi_2)\trans{\ahist_2'}(\alocation_3,\varphi_2)
		\ .
		\label[property]{proof:unpealing:closure}
	\end{align}
	Then, there is $\alocation_1,\varphi_1,\agenheap',\anevent_1$ with:
	\begin{align}
		\alocation_1\in\lreachof{\athread}{\anadr}{H}
		\quad\text{and}\quad
		\agenheap'(\apavar)=\varphi_1(\anovarp)
		\quad\text{and}\quad
		\anevent_1=\evalcom{\agenheap'}{\varphi_1(\anovar)}{\acom}
		\quad\text{and}\quad
		(\alocation_1,\varphi_1)\trans{\anevent_1}(\alocation_2,\varphi_1)
		\ .
		\label[property]{proof:unpealing:post}
	\end{align}
	And last, there is $\ahist_1,\varphi$ with
	\begin{align}
		\ahist_1\in H
		\quad\text{and}\quad
		\varphi=\set{\anovar\mapsto\athread,\anovarp\mapsto\anadr}
		\quad\text{and}\quad
		(\alocation_\mathit{init},\varphi)\trans{\ahist_1}(\alocation_1,\varphi)
		\label[property]{proof:unpealing:reach}
	\end{align}
	where $\alocation_\mathit{init}$ is the initial location in $\anobs$.
	Let $\anevent:=\renamingof{\renamingof{\anevent_1}{\varphi_1(\anovar)}{\athread}}{\varphi_1(\anovarp)}{\anadr}$.
	Then, \Cref{proof:unpealing:renaming-vs-runs} together with \Cref{proof:unpealing:post} gives:
	\begin{align*}
		(\alocation_1,\varphi)\trans{\anevent}(\alocation_2,\varphi)
		\ .
	\end{align*}
	Now, let $\ahist_2:=\renamingof{\renamingof{\anevent_2'}{\varphi_2(\anovar)}{\athread}}{\varphi_2(\anovarp)}{\anadr}$.
	Then, \Cref{proof:unpealing:renaming-vs-runs} together with \Cref{proof:unpealing:closure} gives:
	\begin{align*}
		\project{\ahist_2}{\athread}=\epsilon
		\quad\text{and}\quad
		(\alocation_2,\varphi)\trans{\ahist_2}(\alocation_3,\varphi)
		\ .
	\end{align*}
	Choose $\agenheap:=\renamingof{\renamingof{\agenheap'}{\varphi_1(\anovar)}{\athread}}{\varphi_1(\anovarp)}{\anadr}$.
	That is $\agenheap(\apavarp)=\renamingof{\renamingof{(\agenheap'(\apavarp))}{\varphi_1(\anovar)}{\athread}}{\varphi_1(\anovarp)}{\anadr}$ for all $\apavarp$.
	Consequently, $\anevent=\evalcom{\agenheap}{\athread}{\acom}$ due to \Cref{proof:unpealing:post}.
	Moreover, $\agenheap(\apavar)=\anadr$ by choice of $\agenheap$ together with \Cref{proof:unpealing:post}.
	This concludes the claim.
\end{proof}

\begin{proof}[Proof of \Cref{thm:gactive-through-locations}]
	Consider $\ahist,\ahistp,\anevent,\athread,\anadr$ with $\set{\ahist,\ahist.\anevent,\ahistp}\subseteq\typehistof{\athread}{\anadr}{\gactive}$.
	Let $\alocation\in\lreachof{\athread}{\anadr}{\set{\ahist}}$ and $\alocation\in\lreachof{\athread}{\anadr}{\set{\ahistp}}$.
	Let $\varphi=\set{\anovar\mapsto\athread,\anovarp\mapsto\anadr}$.
	This means there is $\alocationp$ such that we have:
	\begin{align*}
		(\alocation_\mathit{init},\varphi)\trans{\ahist}(\alocation,\varphi)\trans{\anevent}(\alocationp,\varphi)
		\qquad\text{and}\qquad
		(\alocation_\mathit{init},\varphi)\trans{\ahistp}(\alocation,\varphi)
	\end{align*}
	where $\alocation_\mathit{init}$ is the initial location in $\anobs$.
	By definition, $\set{\ahist,\ahistp}\subseteq\typehistof{\athread}{\anadr}{\gactive}$ implies:
	\begin{align*}
		(\ref{obs:base:init},\varphi)\trans{\ahist}(\ref{obs:base:init},\varphi)
		\qquad\text{and}\qquad
		(\ref{obs:base:init},\varphi)\trans{\ahistp}(\ref{obs:base:init},\varphi)
		\ .
	\end{align*}
	Together with $\ahist.\anevent\in\typehistof{\athread}{\anadr}{\gactive}$ we get:
	\begin{align*}
		(\ref{obs:base:init},\varphi)\trans{\ahist}(\ref{obs:base:init},\varphi)\trans{\anevent}(\ref{obs:base:init},\varphi)
		\ .
	\end{align*}
	That is, the following holds:
	\begin{align*}
		(\ref{obs:base:init},\varphi)\trans{\ahistp}(\ref{obs:base:init},\varphi)\trans{\anevent}(\ref{obs:base:init},\varphi)
	\end{align*}
	This means that $\ahistp.\anevent\in\typehistof{\athread}{\anadr}{\gactive}$ holds.
	This concludes the claim.
\end{proof}

\begin{proof}[Proof of \Cref{thm:glocal-through-locations}]
	Follows from \Cref{thm:gactive-through-locations} because $\typehistof{\athread}{\anadr}{\gactive}=\typehistof{\athread}{\anadr}{\glocal}$ for all $\athread,\anadr$ by \Cref{thm:closure-local}.
\end{proof}

\begin{proof}[Proof of \Cref{thm:gsafeaccess-through-locations}]
	Consider $\ahist,\ahistp,\athread,\anadr$ with $\ahist\in\typehistof{\athread}{\anadr}{\gsafeaccess}$.
	Let $\alocation\in\lreachof{\athread}{\anadr}{\set{\ahist}}\cap\lreachof{\athread}{\anadr}{\set{\ahistp}}$.
	Let $\varphi=\set{\anovar\mapsto\athread,\anovarp\mapsto\anadr}$.
	This means we have:
	\begin{align*}
		(\alocation_\mathit{init},\varphi)\trans{\ahist}(\alocation,\varphi)
		\qquad\text{and}\qquad
		(\alocation_\mathit{init},\varphi)\trans{\ahistp}(\alocation,\varphi)
	\end{align*}
	where $\alocation_\mathit{init}$ is the initial location in $\anobs$.
	To arrive at $\ahistp\in\typehistof{\athread}{\anadr}{\gsafeaccess}$, we need to find some set of histories $H$ such that $\extclosureof{\athread}{H}=H$, $\ahistp\in H$ and $\ahistpp\in H\implies\ahistpp.\freeof{\anadr}\notin\specof{\anobs}$.
	We choose $H=\setcond{\ahistp.\ahistpp}{\project{\ahistpp}{\athread}=\epsilon}$.
	Then, $\extclosureof{\athread}{H}=H$ and $\ahistp\in H$ are satisfied.
	So consider some arbitrary $\ahistpp$ with $\project{\ahistpp}{\athread}=\epsilon$.
	Note that $\ahistp.\ahistpp\in H$.
	We show that $\ahistp.\ahistpp.\freeof{\anadr}\notin\specof{\anobs}$ holds.

	To see this, recall $\ahist\in\typehistof{\athread}{\anadr}{\gsafeaccess}$.
	That is, there is some $H'\subseteq\typehistof{\athread}{\anadr}{\gsafeaccess}$ with $\extclosureof{\athread}{H'}=H'$ and $\ahist\in H'$.
	By definition, $\ahist.\ahistpp\in H'$ and thus $\ahist.\ahistpp\in\typehistof{\athread}{\anadr}{\gsafeaccess}$.
	Let $\alocationp$ be a location with:
	\begin{align*}
		(\alocation_\mathit{init},\varphi)\trans{\ahist}(\alocation,\varphi)\trans{\ahistpp.\freeof{\anadr}}(\alocationp,\varphi)
	\end{align*}
	Then, \Cref{assumption:isprotected-reach-new-new} states that $\alocationp$ is final in $\anobs$.
	Moreover, we get:
	\begin{align*}
		(\alocation_\mathit{init},\varphi)\trans{\ahistp}(\alocation,\varphi)\trans{\ahistpp.\freeof{\anadr}}(\alocationp,\varphi)
	\end{align*}
	by assumption.
	This means $\ahistp.\ahistpp.\freeof{\anadr}\notin\specof{\anobs}$ as desired.
	This concludes the claim.
	%
	% By definition of $\typehistof{\athread}{\anadr}{\gsafeaccess}$,
	% Now, $\ahist\in\typehistof{\athread}{\anadr}{\gsafeaccess}$ together with \Cref{assumption:isprotected-reach-new} implies:
	% \begin{align*}
	% 	\forall\ahistpp\;\exists\alocationp.~~
	% 	\project{\ahistpp}{\athread}=\epsilon
	% 	\implies
	% 	(\alocation_\mathit{init},\varphi)
	% 	\trans{\ahist}
	% 	(\alocation,\varphi)
	% 	\trans{\ahistpp.\freeof{\anadr}}
	% 	(\alocationp,\varphi)
	% 	\wedge
	% 	\alocationp\text{ final}
	% 	\ .
	% \end{align*}
	% Then, we get
	% \begin{align*}
	% 	\forall\ahistpp\;\exists\alocationp.~~
	% 	\project{\ahistpp}{\athread}=\epsilon
	% 	\implies
	% 	(\alocation_\mathit{init},\varphi)
	% 	\trans{\ahistp}
	% 	(\alocation,\varphi)
	% 	\trans{\ahistpp.\freeof{\anadr}}
	% 	(\alocationp,\varphi)
	% 	\wedge
	% 	\alocationp\text{ final}
	% 	\ .
	% \end{align*}
	% From \Cref{assumption:isprotected-reach} we get $\ahistp\in\typehistof{\athread}{\anadr}{\gsafeaccess}$.
	% This concludes the claim.
\end{proof}

\begin{proof}[Proof of \Cref{thm:most-precise-mimicks-inference}]
	Let $\aninstantiation,\aninstantiationp$ be two type instantiations.
	Let $\aninstantiationp$ be most precise according to \Cref{def:mostprecise-new}.
	Let $\envi_1,\envi_2\envfrom\aninstantiation$ and $\env_1\envfrom\aninstantiationp$ with $\checkof[\aninstantiation]{\envi_1}{\acom}{\envi_2}$ and $\envi_1\lessprecise\env_1$.
	Consider some arbitrary $\apavar\in\pvars\cup\gvars$.
	% Consider some arbitrary thread $\athread$, valuation $\psi$, and $\lambda\in\pvars\cup\gvars$\todo{$\gvars$ defined?}.
	% Let $\anadr:=\psi(\lambda)$ and let $\anevent:=\psi_\athread(\acom)$.
	From \Cref{def:mostprecise-new} for $\env_1(\apavar),\apavar,\acom$ we get some $\atype\subseteq\aninstantiationp$ with:
	\begin{align}
		\forall\athread,\anadr.~&
		\lreachof{\athread}{\anadr}{\typehistof{\athread}{\anadr}{\atype}}
		=
		\lclosureof{\lpostof{\apavar}{\acom}{\lreachof{\athread}{\anadr}{\typehistof{\athread}{\anadr}{\env_1(\apavar)}}}}
		\label[property]{proof:most-precise-mimicks-inference:synth-type}
		\\\text{and}\qquad
		\forall\athread,\anadr,\ahist.~&
		\lreachof{\athread}{\anadr}{\typehistof{\athread}{\anadr}{\atype}}
		\cap
		\lreachof{\athread}{\anadr}{\set{\ahist}}
		\neq\emptyset
		\implies
		\ahist\in\typehistof{\athread}{\anadr}{\atype}
		\label[property]{proof:most-precise-mimicks-inference:synth-location}
		\ .
	\end{align}
	Then, we choose $\env_2(\apavar)$ as follows:
	\begin{align}
		\env_2(\apavar) := \atype \cup \atypep
		\qquad\text{where}\qquad
		\atypep = \envi_2(\apavar)\cap\set{\gactive,\glocal,\gsafeaccess}
		\ .
	\end{align}

	First, we show that $\envi_2(\apavar)\lessprecise\env_2(\apavar)$ holds.
	We have $\envi_2(\apavar)\cap\set{\gactive,\glocal,\gsafeaccess}=\env_2(\apavar)\cap\set{\gactive,\glocal,\gsafeaccess}$ due to the choice of $\env_2(\apavar)$.
	Consider now some arbitrary thread $\athread$ and some arbitrary address $\anadr$.
	Let $\alocation\in\lreachof{\athread}{\anadr}{\typehistof{\athread}{\anadr}{\env_2(\apavar)\setminus\set{\gactive,\glocal,\gsafeaccess}}}$.
	Note that we have $\alocation\in\lreachof{\athread}{\anadr}{\typehistof{\athread}{\anadr}{\atype}}$ by choice of $\env_2(\apavar)$.
	We show that this implies the desired $\alocation\in\lreachof{\athread}{\anadr}{\typehistof{\athread}{\anadr}{\envi_2(\apavar)\setminus\set{\gactive,\glocal,\gsafeaccess}}}$.
	To see this, we apply \Cref{proof:most-precise-mimicks-inference:synth-type} to $\alocation\in\lreachof{\athread}{\anadr}{\typehistof{\athread}{\anadr}{\atype}}$ and get: \[
		\alocation\in\lclosureof{\lpostof{\apavar}{\acom}{\lreachof{\athread}{\anadr}{\typehistof{\athread}{\anadr}{\env_1(\apavar)}}}}
		\ .
	\]
	By \Cref{thm:unpealing} there are some $\alocation_1,\alocation_2,\varphi,\agenheap,\ahist_1,\ahist_2,\anevent$ with:
	\begin{align*}
		&\alocation_1\in\lreachof{\athread}{\anadr}{\typehistof{\athread}{\anadr}{\env_1(\apavar)}}
		\quad\text{and}\quad
		\anevent=\evalcom{\agenheap}{\athread}{\acom}
		\quad\text{and}\quad
		% \agenheap(\apavar)=\anadr
		\quad\text{and}\quad
		\project{\ahist_2}{\athread}=\epsilon
		\\\text{and}\quad
		&\varphi=\set{\anovar\mapsto\athread,\anovarp\mapsto\anadr}
		\quad\text{and}\quad
		(\alocation_\mathit{init},\varphi)\trans{\ahist_1}(\alocation_1,\varphi)\trans{\anevent}(\alocation_2,\varphi)\trans{\ahist_2}(\alocation,\varphi)
		\\\text{and}\quad
		&\apavar\in\pvars\implies\anadr=\agenheap(\apavar)
		\quad\text{and}\quad
		\apavar\in\gvars\implies\anadr\in\agenheap(\apavar)
	\end{align*}
	where $\alocation_\mathit{init}$ is the initial location in $\anobs$.
	Due to $\envi_1\lessprecise\env_1$ together with \Cref{thm:lessprecise-reach-inclusion} we have $\alocation_1\in\lreachof{\athread}{\anadr}{\typehistof{\athread}{\anadr}{\envi_1(\apavar)}}$.
	So there is some $\ahistp_1\in\typehistof{\athread}{\anadr}{\envi_1(\apavar)}$ such that:
	\begin{align*}
		(\alocation_\mathit{init},\varphi)\trans{\ahistp_1}(\alocation_1,\varphi)\trans{\anevent}(\alocation_2,\varphi)\trans{\ahist_2}(\alocation,\varphi)
		\ .
	\end{align*}
	Now, we get $\ahistp_1.\anevent\in\typehistof{\athread}{\anadr}{\envi_2(\apavar)}$ from $\checkof[\aninstantiation]{\envi_1}{\acom}{\envi_2}$.
	Let $G=\envi_2(\apavar)\setminus\set{\gactive,\glocal,\gsafeaccess}$.
	By definition, we have $\ahistp_1.\anevent\in\typehistof{\athread}{\anadr}{G}$.
	To establish the desired $l\in\lreachof{\athread}{\anadr}{\typehistof{\athread}{\anadr}{G}}$, it suffices to establish $\ahistp_1.\anevent.\ahist_2\in\typehistof{\athread}{\anadr}{G}$.
	If $G=\emptyset$, this follows from $\typehistof{\athread}{\anadr}{\emptyset}$ containing all histories by definition.
	Otherwise, $G\neq\emptyset$.
	Let $\aguarantee\in G$ be some arbitrary guarantee from $G$.
	By definition, $\ahistp_1.\anevent\in\typehistof{\athread}{\anadr}{\aguarantee}$.
	Note that $\aguarantee$ is a user-specified guarantee, that is, $\aguarantee\notin\set{\gactive,\glocal,\gsafeaccess}$.
	Since $\aguarantee$ must satisfy the non-interference property (\Cref{eq:types:non-interference}), $\ahistp_1.\anevent.\ahist_2\in\typehistof{\athread}{\anadr}{\aguarantee}$ follows from $\project{\ahist_2}{\athread}=\epsilon$ together with \Cref{eq:types:non-interference}.
	Altogether, we get the desired $\ahistp_1.\anevent.\ahist_2\in\typehistof{\athread}{\anadr}{G}$.
	This concludes $\envi_2(\apavar)\lessprecise\env_2(\apavar)$.

	\medskip
	Second, we show that $\checkof[\aninstantiationp]{\env_1}{\acom}{\env_2}$ holds.
	We focus on the case for some arbitrary $\apavar$.
	Therefore, consider some arbitrary thread $\athread$ and valuation $\agenheap$.
	Let $\anadr=\agenheap(\apavar)$ and $\anevent:=\evalcom{\agenheap}{\athread}{\acom}$.
	We have:
	\begin{align*}
		\gactive\in\env_2(\apavar)
		\implies
		\gactive\in\envi_2(\apavar)
		\implies
		\gactive\in\envi_1(\apavar)
		\implies
		\gactive\in\env_1(\apavar)
	\end{align*}
	where the first implication is due to the above $\envi_2\lessprecise\env_2$, the second implication is due to the premise $\checkof[\aninstantiation]{\envi_1}{\acom}{\envi_2}$, and the last implication is due to the premise $\envi_1\lessprecise\env_1$ .
	Similarly, we conclude that $\glocal\in\env_2(\apavar)\implies\glocal\in\env_1(\apavar)$ and $\isvalidof{\env_2(\apavar)}\implies\isvalidof{\env_1(\apavar)}$ hold.

	Consider now $\ahist\in\typehistof{\athread}{\anadr}{\env_1(\apavar)}$.
	We show that $\ahist.\anevent\in\typehistof{\athread}{\anadr}{\env_2(\apavar)}$.
	As a first step, we show that $\ahist.\anevent\in\typehistof{\athread}{\anadr}{\atype}$.
	Let $\alocation\in\lreachof{\athread}{\anadr}{\set{\ahist}}$.
	Note that this means $\alocation\in\lreachof{\athread}{\anadr}{\typehistof{\athread}{\anadr}{\env_1(\apavar)}}$.
	Let $\alocationp$ be a location such that $(\alocation,\varphi)\trans{\anevent}(\alocationp,\varphi)$.
	By definition, we have $\alocationp\in\lpostof{\apavar}{\acom}{\lreachof{\athread}{\anadr}{\typehistof{\athread}{\anadr}{\env_1(\apavar)}}}$.
	So:
	\begin{align*}
		\alocationp\in\lclosureof{\lpostof{\apavar}{\acom}{\lreachof{\athread}{\anadr}{\typehistof{\athread}{\anadr}{\env_1(\apavar)}}}}
		\ .
	\end{align*}
	From \Cref{proof:most-precise-mimicks-inference:synth-type} we get $\alocationp\in\lreachof{\athread}{\anadr}{\typehistof{\athread}{\anadr}{\atype}}$.
	Moreover, we have $\alocationp\in\lreachof{\athread}{\anadr}{\set{\ahist.\anevent}}$ by the choice of $\alocationp$.
	That is, $\lreachof{\athread}{\anadr}{\typehistof{\athread}{\anadr}{\atype}}\cap\lreachof{\athread}{\anadr}{\set{\ahist.\anevent}}\neq\emptyset$.
	Hence, \Cref{proof:most-precise-mimicks-inference:synth-location} gives the desired $\ahist.\anevent\in\typehistof{\athread}{\anadr}{\atype}$.

	It remains to show that $\ahist.\anevent\in\typehistof{\athread}{\anadr}{\atypep}$.
	If $\atypep=\emptyset$, this holds by definition.
	Otherwise, $\atypep\neq\emptyset$.
	Let $\aguarantee\in\atypep$ be some guarantee from $\atypep$.
	Note that $\aguarantee\in\set{\gactive,\glocal,\gsafeaccess}$.
	We do a case distinction on $\aguarantee$.
	\begin{compactitem}
		\item
			Consider the case $\aguarantee=\gactive$.
			Recall from above: $\alocation\in\lreachof{\athread}{\anadr}{\typehistof{\athread}{\anadr}{\set{\ahist}}}\cap\lreachof{\athread}{\anadr}{\typehistof{\athread}{\anadr}{\env_1(\apavar)}}$.
			From $\envi\lessprecise\env$ together with \Cref{thm:lessprecise-reach-inclusion} we get $\alocation\in\lreachof{\athread}{\anadr}{\typehistof{\athread}{\anadr}{\envi_1(\apavar)}}$.
			That is, there is some $\ahistp\in\typehistof{\athread}{\anadr}{\envi_1(\apavar)}$ with $\alocation\in\lreachof{\athread}{\anadr}{\typehistof{\athread}{\anadr}{\set{\ahistp}}}$.
			By $\checkof[\aninstantiation]{\envi_1}{\acom}{\envi_2}$, we have $\ahistp.\anevent\in\typehistof{\athread}{\anadr}{\envi_2(\apavar)}$.
			Moreover, we have $\gactive\in\envi_2(\apavar)$ by choice of $\atypep$ and thus $\gactive\in\envi_1(\apavar)$ by $\checkof[\aninstantiation]{\envi_1}{\acom}{\envi_2}$.
			This means $\ahistp\in\typehistof{\athread}{\anadr}{\gactive}$ and $\ahistp.\anevent\in\typehistof{\athread}{\anadr}{\gactive}$.
			And from $\envi_1\lessprecise\env_1$ we get $\gactive\in\env_1(\apavar)$.
			So we can invoke \Cref{thm:gactive-through-locations}.
			It yields $\ahist.\anevent\in\typehistof{\athread}{\anadr}{\gactive}$.
		\item
			Consider the case $\aguarantee=\glocal$.
			This case is analogous to the previous one, except for that fact that it uses \Cref{thm:glocal-through-locations} instead of \Cref{thm:gactive-through-locations}.
		\item
			Consider the $\aguarantee=\gsafeaccess$.
			As in the previous case, there is some history $\ahistp\in\typehistof{\athread}{\anadr}{\envi_1(\apavar)}$ such that $\ahistp.\anevent\in\typehistof{\athread}{\anadr}{\envi_2(\apavar)}$ and $\alocation\in\lreachof{\athread}{\anadr}{\typehistof{\athread}{\anadr}{\set{\ahist}}}\cap\lreachof{\athread}{\anadr}{\typehistof{\athread}{\anadr}{\set{\ahistp}}}$.
			Let $\alocationp$ be some location with $(\alocation,\varphi)\trans{\anevent}(\alocationp,\varphi)$.
			Then, $\alocationp\in\lreachof{\athread}{\anadr}{\typehistof{\athread}{\anadr}{\set{\ahist.\anevent}}}\cap\lreachof{\athread}{\anadr}{\typehistof{\athread}{\anadr}{\set{\ahistp.\anevent}}}$ holds by definition.
			And by choice of $\atypep$, we have $\gactive\in\envi_2(\apavar)$.
			That is, $\ahistp.\anevent\in\typehistof{\athread}{\anadr}{\gactive}$.
			An invocation of \Cref{thm:gsafeaccess-through-locations} then yields $\ahist.\anevent\in\typehistof{\athread}{\anadr}{\gsafeaccess}$.
	\end{compactitem}
	Each case of the above case distinction results in $\ahist.\anevent\in\typehistof{\athread}{\anadr}{\aguarantee}$.
	So we get $\ahist.\anevent\in\typehistof{\athread}{\anadr}{\atypep}$ altogether.
	That is, $\ahist.\anevent\in\typehistof{\athread}{\anadr}{\env_2(\apavar)}$.
	This concludes $\checkof[\aninstantiationp]{\env_1}{\acom}{\env_2}$.
\end{proof}

\begin{proof}[Proof of \Cref{thm:most-precise-mimicks-judgements-com}]
	Let $\envi_1,\envi_2\envfrom\aninstantiation$ and $\acom$ with $\typecom[\aninstantiation]{\envi_1}{\acom}{\envi_2}$.
	Let $\env_1\envfrom\aninstantiationp$ with $\envi_1\lessprecise\env_1$.
	Let $\aninstantiationp$ be most precise according to \Cref{def:mostprecise-new}.
	We show that there is $\env_2\envfrom\aninstantiationp$ such that $\typecom[\aninstantiationp]{\env_1}{\acom}{\env_2}$ and $\envi_2\lessprecise\env_2$.

	First, let the derivation $\typecom[\aninstantiation]{\envi_1}{\acom}{\envi_2}$ be due to any rule except \ref{rule:enter} and \ref{rule:exit}.
	Note that the rule used for the derivation is applicable for $\env_1$ due to $\envi_1\lessprecise\env_1$.
	To see this, observe that $\isvalidof{\envi_1(\lambda)}\iff\isvalidof{\env_1(\lambda)}$ follows for any $\lambda$ from $\envi_1\lessprecise\env_1$.
	The rules yield a determined post environment $\env_2$.
	To obtain $\env_2$, the rules either add/remove guarantees from $\set{\gactive,\glocal,\gsafeaccess}$ or join types.
	The former preservers $\lessprecise$ and gives the desired $\envi_2\lessprecise\env_2$.
	For a type join, consider some $\lambda_1,\lambda_2$ and some $\athread,\anadr$.
	By $\envi_1\lessprecise\env_1$ we have: $\typehistof{\athread}{\anadr}{\env_1(\lambda_i)\setminus\set{\gactive,\glocal,\gsafeaccess}}\subseteq\typehistof{\athread}{\anadr}{\envi_1(\lambda_i)\setminus\set{\gactive,\glocal,\gsafeaccess}}$ and $\envi_1(\lambda_i)\cap\set{\gactive,\glocal,\gsafeaccess}=\env_1(\lambda_i)\cap\set{\gactive,\glocal,\gsafeaccess}$ for $i\in\set{1,2}$.
	We immediately get:
	\begin{align*}
		(\envi_1(\lambda_1)\cup\envi_1(\lambda_2))\cap\set{\gactive,\glocal,\gsafeaccess}&=(\env_1(\lambda_1)\cup\env_1(\lambda_2))\cap\set{\gactive,\glocal,\gsafeaccess}
		\ .
	\intertext{
	Moreover, we have:
	}
		\typehistof{\athread}{\anadr}{(\env_1(\lambda_1)\cup\env_1(\lambda_2))\setminus\set{\gactive,\glocal,\gsafeaccess}}
		&=
		\typehistof{\athread}{\anadr}{(\env_1(\lambda_1)\setminus\set{\gactive,\glocal,\gsafeaccess})\cup(\env_1(\lambda_2)\setminus\set{\gactive,\glocal,\gsafeaccess})}\\
		&=
		\typehistof{\athread}{\anadr}{(\env_1(\lambda_1)\setminus\set{\gactive,\glocal,\gsafeaccess})}
		\cap
		\typehistof{\athread}{\anadr}{(\env_1(\lambda_2)\setminus\set{\gactive,\glocal,\gsafeaccess})}\\
		&\subseteq
		\typehistof{\athread}{\anadr}{(\envi_1(\lambda_1)\setminus\set{\gactive,\glocal,\gsafeaccess})}
		\cap
		\typehistof{\athread}{\anadr}{(\envi_1(\lambda_2)\setminus\set{\gactive,\glocal,\gsafeaccess})}\\
		&=
		\typehistof{\athread}{\anadr}{(\envi_1(\lambda_1)\setminus\set{\gactive,\glocal,\gsafeaccess})\cup(\envi_1(\lambda_2)\setminus\set{\gactive,\glocal,\gsafeaccess})}\\
		&=
		\typehistof{\athread}{\anadr}{(\envi_1(\lambda_1)\cup\envi_1(\lambda_2))\setminus\set{\gactive,\glocal,\gsafeaccess}}
		\ .
	\end{align*}
	From this we conclude $\envi_2\lessprecise\env_2$.

	Second, consider the case where $\typecom[\aninstantiation]{\envi_1}{\acom}{\envi_2}$ is due to Rule~\ref{rule:enter}.
	As before, we have $\isvalidof{\envi_1(\lambda)}\iff\isvalidof{\env_1(\lambda}$.
	Hence, $\safecallof{\envi}{\afuncof{\vecof{\apvar},\vecof{\advar}}}\iff\safecallof{\env}{\afuncof{\vecof{\apvar},\vecof{\advar}}}$.
	So the rule is also enabled in $\env_1$.
	The post type environment $\env_2$ is obtained by type inference.
	By \Cref{thm:most-precise-mimicks-inference} an appropriate such $\env_2$ exists.

	Last, consider consider the case where $\typecom[\aninstantiation]{\envi_1}{\acom}{\envi_2}$ is due to Rule~\ref{rule:exit}.
	Desired result follows analogously to Rule~\ref{rule:enter}.
\end{proof}

\begin{proof}[Proof of \Cref{thm:most-precise-mimicks-judgements-stmt}]
	We do an induction on the depth of the derivation of $\typestmt[\aninstantiation]{\envi_1}{\astmt}{\envi_2}$.
	\begin{description}[labelwidth=6mm,leftmargin=8mm,itemindent=0mm]
		\item[IB:]
			The derivation $\typestmt[\aninstantiation]{\envi_1}{\astmt}{\envi_2}$ is due to one of the following rules: \ref{rule:com}, \ref{rule:begin}, or \ref{rule:end}.
			For Rule~\ref{rule:com} the claim follows from \Cref{thm:most-precise-mimicks-judgements-com}.
			For Rule~\ref{rule:begin} the claim follows immediately by choosing $\env_2:=\env_1$.
			For Rule~\ref{rule:begin} we choose $\env_2:=\rmtransientof{\env_1}$.
			To see that this gives $\envi_2\lessprecise\env_2$, consider some $\athread,\anadr,\lambda$.
			If $\lambda\in\svars$, then $\envi_2(\lambda)=\env_2(\lambda)$.
			Otherwise, we have $\envi_2(\lambda)=\envi_1(\lambda)\setminus\set{\gactive}$ and $\env_2(\lambda)=\env_1(\lambda)\setminus\set{\gactive}$.
			Then, \Cref{thm:lessprecise-vs-gactive-removal} together with $\envi_1\lessprecise\env_1$ gives $\envi_2\lessprecise\env_2$.
			This concludes the desired $\typestmt[\aninstantiationp]{\env_1}{\astmt}{\env_2}$.

		\item[IH:]
			The claim holds for all derivations $\typestmt[\aninstantiation]{\envi_1}{\astmt}{\envi_2}$ up to depth $n$.

		\item[IS:]
			Consider a derivation $\typestmt[\aninstantiation]{\envi_1}{\astmt}{\envi_4}$ of depth $n+1$.
			The topmost rule is one of: \ref{rule:infer}, \ref{rule:seq}, \ref{rule:choice}, or \ref{rule:loop}.

			First, consider Rule~\ref{rule:infer}.
			We have $\checkof[\aninstantiation]{\envi_1}{\epsilon}{\envi_2}$, $\typestmt[\aninstantiation]{\envi_2}{\astmt}{\envi_3}$, and $\checkof[\aninstantiation]{\envi_3}{\epsilon}{\envi_4}$.
			From \Cref{thm:most-precise-mimicks-inference} for $\envi_1$ and $\env_1$ we get $\env_2$ with $\envi_2\lessprecise\env_2$ and $\checkof[\aninstantiationp]{\env_1}{\epsilon}{\env_2}$.
			By induction, this yields $\env_3$ with $\envi_3\lessprecise\env_3$ and $\typestmt[\aninstantiationp]{\env_2}{\astmt}{\env_3}$.
			Again by \Cref{thm:most-precise-mimicks-inference}, we get $\env_4$ with $\envi_4\lessprecise\env_4$ and $\checkof[\aninstantiationp]{\env_3}{\epsilon}{\env_4}$.
			Together, this means $\typestmt[\aninstantiationp]{\env_1}{\astmt}{\env_4}$.
			This concludes the claim for Rule~\ref{rule:infer}.

			Second, consider Rule~\ref{rule:seq}.
			Then, $\astmt$ is of the form $\astmt\equiv\astmt_1;\astmt_2$.
			Moreover, we have $\typestmt[\aninstantiation]{\envi_1}{\astmt_1}{\envi_2}$ and $\typestmt[\aninstantiation]{\envi_2}{\astmt_2}{\envi_4}$.
			By induction, there is $\env_2$ with $\envi_2\lessprecise\env_2$ and $\typestmt[\aninstantiationp]{\env_1}{\astmt_1}{\env_2}$.
			Then, we can apply induction again and get $\env_4$ with $\envi_4\lessprecise\env_4$ and $\typestmt[\aninstantiationp]{\env_2}{\astmt_2}{\env_4}$.
			Together, this means $\typestmt[\aninstantiationp]{\env_1}{\astmt}{\env_4}$.
			This concludes the claim for Rule~\ref{rule:seq}.

			The remaining rules are analogous to the one for Rule~\ref{rule:seq}.
			% Last, consider Rules~\ref{rule:choice} and \ref{rule:loop}.
			% The reasoning is analogous to the one for Rule~\ref{rule:seq}.
	\end{description}
	The induction concludes the claim.
\end{proof}

\begin{proof}[Proof of \Cref{thm:most-precise-mimicks-typecheck}]
	Consider $\aninstantiation,\aninstantiationp$ and $\aprog$ with $\typechecks[\aninstantiation]{\aprog}$.
	Let $\aninstantiationp$ be most precise according to \Cref{def:mostprecise-new}.
	The fact that we have $\typechecks[\aninstantiation]{\aprog}$ means that there is some type environment $\envi$ such that $\typestmt[\aninstantiation]{\envinit}{\aprog}{\envi}$.
	Note that $\envinit\envfrom\aninstantiation$ and $\envinit\envfrom\aninstantiationp$ holds.
	Moreover, $\envinit\lessprecise\envinit$ by definition.
	So an invocation of \Cref{thm:most-precise-mimicks-judgements-stmt} yields some $\env\envfrom\aninstantiationp$ with $\typestmt[\aninstantiationp]{\envinit}{\aprog}{\env}$.
	So $\typechecks[\aninstantiationp]{\aprog}$ holds as desired.
\end{proof}

\begin{proof}[Proof of \Cref{thm:synthesized-types-are-most-precise-new}]
	Let $\smrobs$ be deterministic.
	Let $\aninstantiationp=\setcond{\gcustom{L}}{L\subseteq\lsetset}$ be the synthesized type system instantiation from \Cref{sec:synthesis}.
	We show that $\aninstantiationp$ is most precise according to \Cref{def:mostprecise-new}.
	To that end, consider some $\atype\typefrom\aninstantiationp$ and some $\lambda,\acom$.
	Let:
	\begin{align*}
		L=\lreachof{\athread}{\anadr}{\typehistof{\athread}{\anadr}{\atype}}
		\qquad\text{and}\qquad
		L'=\lclosureof{\lpostof{\lambda}{\acom}{L}}
		\ .
	\end{align*}
	Note that $\gcustom{L'}\in\aninstantiationp$.
	We show that $\gcustom{L'}$ satisfies the requirements.
	\begin{compactitem}
		\item
			Let $\alocation\in L'$.
			From \Cref{thm:unpealing} we get the following run on $\smrobs$:
			\begin{align*}
				(\alocation_\mathit{init},\varphi)\trans{\ahist_1}(\alocation_1,\varphi)\trans{\anevent}(\alocation_2,\varphi)\trans{\ahist_2}(\alocation,\varphi)
			\end{align*}
			for some history $\ahist_1.\anevent.\ahist_2$ and $\varphi=\set{\anovar\mapsto\athread,\anovarp\mapsto\anadr}$.
			That is, $\alocation\in\lreachof{\athread}{\anadr}{\set{\ahist_1.\anevent.\ahist_2}}$.
			Hence, $\lreachof{\athread}{\anadr}{\set{\ahist_1.\anevent.\ahist_2}}\cap L'\neq\emptyset$.
			So we have $\ahist_1.\anevent.\ahist_2\in\typehistof{\athread}{\anadr}{\gcustom{L'}}$.
			This means the desired $\alocation\in\lreachof{\athread}{\anadr}{\typehistof{\athread}{\anadr}{\gcustom{L'}}}$ holds.
		\item
			Let $\alocation\in\lreachof{\athread}{\anadr}{\typehistof{\athread}{\anadr}{\gcustom{L'}}}$.
			By definition, there is $\ahist\in\typehistof{\athread}{\anadr}{\gcustom{L'}}$ with $\alocation\in\lreachof{\athread}{\anadr}{\set{\ahist}}$.
			Moreover, there is $\alocationp\in L'$ with $\alocationp\in\lreachof{\athread}{\anadr}{\set{\ahist}}$ by the definition of the induced histories $\typehistof{\athread}{\anadr}{\gcustom{L'}}$.
			Since $\smrobs$ is assumed to be deterministic, we get $\set{\alocationp}=\lreachof{\athread}{\anadr}{\set{\ahist}}$.
			Hence, $\alocation=\alocationp$ must hold.
			This gives the desired $\alocation\in L'$.
		\item
			Let $\alocation\in\lreachof{\athread}{\anadr}{\typehistof{\athread}{\anadr}{\gcustom{L'}}}\cap\lreachof{\athread}{\anadr}{\set{\ahist}}$.
			From the above, we know that $\alocation\in L'$ holds.
			Hence, $\ahist\in\typehistof{\athread}{\anadr}{\gcustom{L'}}$ follows by definition.
	\end{compactitem}
	Altogether, this establishes the requirements of \Cref{def:mostprecise-new} and shows that $\aninstantiationp$ is indeed a most precise type system instantiation.
\end{proof}

\begin{proof}[Proof of \Cref{thm:synthesized-types-mimic-all-types-new}]
	Follows from \Cref{thm:most-precise-mimicks-typecheck,thm:synthesized-types-are-most-precise-new}.
\end{proof}

\begin{proof}[Proof of \Cref{thm:synthesized-guarantees-are-closed-under-interference}]
	Let $\gcustom{L}$ be some synthesized guarantee with $L=\lclosureof{L}$.
	We show that $\gcustom{L}$ satisfies \Cref{eq:types:non-interference}.
	To that end, consider some $\athread,\anadr,\ahist.\ahistp$ with $\ahist\in\typehistof{\athread}{\anadr}{\gcustom{L}}$ and $\project{\ahistp}{\athread}=\epsilon$.
	By definition of $\gcustom{L}$, there is $\alocation\in L$ with $\alocation\in\lreachof{\athread}{\anadr}{\set{\ahist}}$.
	Let $\varphi=\set{\anovar\mapsto\athread,\anovarp\mapsto\anadr}$.
	Let $\alocationp$ be some location with $(\alocation,\varphi)\trans{\ahistp}(\alocationp,\varphi)$.
	By definition, $\alocationp\in\lclosureof{\set{\ahist}}$.
	Hence, $\alocationp\in L$ due to the premise.
	Note that $\alocationp\in\lreachof{\athread}{\anadr}{\set{\ahist.\ahistp}}$.
	Hence, the definition of the induced histories of $\gcustom{L}$ gives the desired $\ahist.\ahistp\in\typehistof{\athread}{\anadr}{\gcustom{L}}$.
\end{proof}
