# Supplementary material for: Pointer Life Cycle Types for Lock-Free Data Structures with Memory Reclamation
Source: arXiv:1910.11714 source file (2019-11-26)
Supplement: Supplementary file 5 [file obs2nfa.tex]

%!TEX root = ../main.tex

\presection
\subsection{Observer to NFA}

\begin{lemma}
	\label{thm:nonempty-history-concretisation}
	Consider some $\anobs,\varphi$.
	Let $\ahist^\sharp\in\langof{\alpha(\anobs)}$.
	Then there is $\ahist$ such that $\ahist^\sharp=\alpha_\varphi(\ahist)$.
\end{lemma}

\begin{lemma}
	\label{thm:concrete-vs-abstract-induced-histories}
	Let $\varphi=\set{\anovar\mapsto\athread,\anovarp\mapsto\anadr}$.
	Consider some type $\atype=\set{\aguarantee_1,\dots,\aguarantee_k}$ and observers $\anobs[1],\dots,\anobs[k]$ with $\typehistof{\athread}{\anadr}{\aguarantee_i}=\setcond{\ahist}{\exists\alocation_1,\alocation_2.~(\alocation_1,\varphi)\trans{\ahist}(\alocation_2,\varphi)\text{ with $\alocation_1$ initial and $\alocation_2$ final in $\anobs[i]$}}$.
	Then, for every history $\ahist$, we have $\ahist\in\typehistof{\athread}{\anadr}{\atype}$ iff\, $\alpha_\varphi(\ahist)\in\langof{\alpha(\anobs[1])\times\cdots\times\alpha(\anobs[k])}$.
\end{lemma}
